# Supplementary material for: Search for sterile neutrinos in MINOS and MINOS+ using a two-detector fit
Source: arXiv:1710.06488 ancillary file (2020-06-03)
Supplement: Supplementary file 1 [file minosSterileSuppMaterials.pdf]

# Search for sterile neutrinos in MINOS and MINOS+ using a two-detector fit: Supplemental discussion

P. Adamson,<sup>8</sup> I. Anghel,<sup>15,1</sup> A. Aurisano,<sup>7</sup> G. Barr,<sup>22</sup> M. Bishai,<sup>3</sup> A. Blake,<sup>5,16</sup> G. J. Bock,<sup>8</sup> D. Bogert,<sup>8</sup> S. V. Cao,<sup>30</sup> T. J. Carroll,<sup>30</sup> C. M. Castromonte,<sup>9</sup> R. Chen,<sup>18</sup> S. Childress,<sup>8</sup> J. A. B. Coelho,<sup>31</sup> L. Corwin,<sup>14,\*</sup> D. Cronin-Hennessy,<sup>19</sup> J. K. de Jong,<sup>22</sup> S. De Rijck,<sup>30</sup> A. V. Devan,<sup>33</sup> N. E. Devenish,<sup>28</sup> M. V. Diwan,<sup>3</sup> C. O. Escobar,<sup>6</sup> J. J. Evans,<sup>18</sup> E. Falk,<sup>28</sup> G. J. Feldman,<sup>10</sup> W. Flanagan,<sup>30</sup> M. V. Frohne,<sup>11,†</sup> M. Gabrielyan,<sup>19</sup> H. R. Gallagher,<sup>31</sup> S. Germani,<sup>17</sup> R. A. Gomes,<sup>9</sup> M. C. Goodman,<sup>1</sup> P. Gouffon,<sup>25</sup> N. Graf,<sup>23</sup> R. Gran,<sup>20</sup> K. Grzelak,<sup>32</sup> A. Habig,<sup>20</sup> S. R. Hahn,<sup>8</sup> J. Hartnell,<sup>28</sup> R. Hatcher,<sup>8</sup> A. Holin,<sup>17</sup> J. Huang,<sup>30</sup> J. Hylen,<sup>8</sup> G. M. Irwin,<sup>27</sup> Z. Ivan,<sup>3</sup> C. James,<sup>8</sup> D. Jensen,<sup>8</sup> T. Kafka,<sup>31</sup> S. M. S. Kasahara,<sup>19</sup> L. W. Koerner,<sup>12</sup> G. Koizumi,<sup>8</sup> M. Kordosky,<sup>33</sup> A. Kreymer,<sup>8</sup> K. Lang,<sup>30</sup> J. Ling,<sup>3</sup> P. J. Litchfield,<sup>19,24</sup> P. Lucas,<sup>8</sup> W. A. Mann,<sup>31</sup> M. L. Marshak,<sup>19</sup> N. Mayer,<sup>31</sup> C. McGivern,<sup>23</sup> M. M. Medeiros,<sup>9</sup> R. Mehdiev,<sup>30</sup> J. R. Meier,<sup>19</sup> M. D. Messier,<sup>14</sup> W. H. Miller,<sup>19</sup> S. R. Mishra,<sup>26</sup> S. Moed Sher,<sup>8</sup> C. D. Moore,<sup>8</sup> L. Muallem,<sup>4</sup> J. Musser,<sup>14</sup> D. Naples,<sup>23</sup> J. K. Nelson,<sup>33</sup> H. B. Newman,<sup>4</sup> R. J. Nichol,<sup>17</sup> J. A. Nowak,<sup>19,‡</sup> J. O'Connor,<sup>17</sup> M. Orchanian,<sup>4</sup> R. B. Pahlka,<sup>8</sup> J. Paley,<sup>1</sup> R. B. Patterson,<sup>4</sup> G. Pawloski,<sup>19</sup> A. Perch,<sup>17</sup> M. M. Pfützner,<sup>17</sup> D. D. Phan,<sup>30</sup> S. Phan-Budd,<sup>1</sup> R. K. Plunkett,<sup>8</sup> N. Poonthottathil,<sup>8</sup> X. Qiu,<sup>27</sup> A. Radovic,<sup>33</sup> B. Rebel,<sup>8</sup> C. Rosenfeld,<sup>26</sup> H. A. Rubin,<sup>13</sup> P. Sail,<sup>30</sup> M. C. Sanchez,<sup>15,1</sup> J. Schneps,<sup>31</sup> A. Schreckenberger,<sup>30</sup> P. Schreiner,<sup>1</sup> R. Sharma,<sup>8</sup> A. Sousa,<sup>7</sup> N. Tagg,<sup>21</sup> R. L. Talaga,<sup>1</sup> J. Thomas,<sup>17</sup> M. A. Thomson,<sup>5</sup> X. Tian,<sup>26</sup> A. Timmons,<sup>18</sup> J. Todd,<sup>7</sup> S. C. Tognini,<sup>9</sup> R. Toner,<sup>10</sup> D. Torretta,<sup>8</sup> G. Tzanakos,<sup>2,†</sup> J. Urheim,<sup>14</sup> P. Vahle,<sup>33</sup> B. Viren,<sup>3</sup> A. Weber,<sup>22,24</sup> R. C. Webb,<sup>29</sup> C. White,<sup>13</sup> L. H. Whitehead,<sup>17,§</sup> S. G. Wojcicki,<sup>27</sup> and R. Zwaska<sup>8</sup>

(The MINOS+ Collaboration)

<sup>1</sup>Argonne National Laboratory, Argonne, Illinois 60439, USA

<sup>2</sup>Department of Physics, University of Athens, GR-15771 Athens, Greece

<sup>3</sup>Brookhaven National Laboratory, Upton, New York 11973, USA

<sup>4</sup>Lauritsen Laboratory, California Institute of Technology, Pasadena, California 91125, USA

<sup>5</sup>Cavendish Laboratory, University of Cambridge, Cambridge CB3 0HE, United Kingdom

<sup>6</sup>Universidade Estadual de Campinas, IFGW, CP 6165, 13083-970, Campinas, SP, Brazil

<sup>7</sup>Department of Physics, University of Cincinnati, Cincinnati, Ohio 45221, USA

<sup>8</sup>Fermi National Accelerator Laboratory, Batavia, Illinois 60510, USA

<sup>9</sup>Instituto de Física, Universidade Federal de Goiás, 74690-900, Goiânia, GO, Brazil

<sup>10</sup>Department of Physics, Harvard University, Cambridge, Massachusetts 02138, USA

<sup>11</sup>Holy Cross College, Notre Dame, Indiana 46556, USA

<sup>12</sup>Department of Physics, University of Houston, Houston, Texas 77204, USA

<sup>13</sup>Department of Physics, Illinois Institute of Technology, Chicago, Illinois 60616, USA

<sup>14</sup>Indiana University, Bloomington, Indiana 47405, USA

<sup>15</sup>Department of Physics and Astronomy, Iowa State University, Ames, Iowa 50011 USA

<sup>16</sup>Lancaster University, Lancaster, LA1 4YB, UK

<sup>17</sup>Department of Physics and Astronomy, University College London, London WC1E 6BT, United Kingdom

<sup>18</sup>School of Physics and Astronomy, University of Manchester, Manchester M13 9PL, United Kingdom

<sup>19</sup>University of Minnesota, Minneapolis, Minnesota 55455, USA

<sup>20</sup>Department of Physics, University of Minnesota Duluth, Duluth, Minnesota 55812, USA

<sup>21</sup>Otterbein University, Westerville, Ohio 43081, USA

<sup>22</sup>Subdepartment of Particle Physics, University of Oxford, Oxford OX1 3RH, United Kingdom

<sup>23</sup>Department of Physics and Astronomy, University of Pittsburgh, Pittsburgh, Pennsylvania 15260, USA

<sup>24</sup>Rutherford Appleton Laboratory, Science and Technology Facilities Council, Didcot, OX11 0QX, United Kingdom

<sup>25</sup>Instituto de Física, Universidade de São Paulo, CP 66318, 05315-970, São Paulo, SP, Brazil

<sup>26</sup>Department of Physics and Astronomy, University of South Carolina, Columbia, South Carolina 29208, USA

<sup>27</sup>Department of Physics, Stanford University, Stanford, California 94305, USA

<sup>28</sup>Department of Physics and Astronomy, University of Sussex, Falmer, Brighton BN1 9QH, United Kingdom

<sup>29</sup>Physics Department, Texas A&M University, College Station, Texas 77843, USA

<sup>30</sup>Department of Physics, University of Texas at Austin, Austin, Texas 78712, USA

<sup>31</sup>Physics Department, Tufts University, Medford, Massachusetts 02155, USA

<sup>32</sup>Department of Physics, University of Warsaw, PL-02-093 Warsaw, Poland

<sup>33</sup>Department of Physics, College of William & Mary, Williamsburg, Virginia 23187, USA

(Dated: February 20, 2019)

# CONTENTS

|                                                                      |    |
|----------------------------------------------------------------------|----|
| I. Introduction                                                      | 2  |
| II. Phenomenology of Sterile Neutrino Oscillations at Long Baselines | 5  |
| III. Systematic Uncertainties                                        | 8  |
| A. Hadron production                                                 | 9  |
| B. Cross Sections                                                    | 11 |
| C. Energy Scale                                                      | 11 |
| D. Beam optics                                                       | 12 |
| E. Acceptance                                                        | 15 |
| F. Effective Normalization Uncertainty                               | 17 |
| IV. Motivation for a Two-Detector Fit                                | 18 |
| V. Mitigation of Correlated Systematic Uncertainties                 | 20 |
| A. Covariance Matrix Fit                                             | 20 |
| B. Systematic Cancellation in the Muon Neutrino CC Sample            | 22 |
| C. Shape vs. Normalization                                           | 23 |
| VI. Degeneracies and Limiting Cases                                  | 24 |
| A. $\Delta m_{41}^2 \rightarrow \infty$                              | 25 |
| B. $\Delta m_{41}^2 = 2\Delta m_{31}^2$                              | 26 |
| C. $\Delta m_{41}^2 = \Delta m_{31}^2$                               | 26 |
| D. $\Delta m_{41}^2 \rightarrow 0$                                   | 27 |
| VII. Limitations of Asimov Sensitivities                             | 27 |
| A. Toy Monte Carlo Studies                                           | 27 |
| B. Fluctuating Systematic Categories                                 | 29 |
| C. Asimov and Median Scaling                                         | 30 |
| VIII. Fitter Assumptions                                             | 32 |
| IX. Results and Discussion                                           | 32 |
| A. Comparison of the Data Limit with Expected Sensitivity            | 33 |
| B. Significance of the FD Neutral Current Excess                     | 34 |
| C. Oscillations at Large Mass Splittings                             | 34 |
| X. Conclusions                                                       | 35 |
| A. Conditional Multivariate Gaussian Distributions                   | 41 |
| 1. Decorrelation Example                                             | 42 |
| References                                                           | 43 |

## I. INTRODUCTION

This document describes the 2017 MINOS and MINOS+ sterile analysis in detail, and it serves as a companion to Ref. [1], which has been submitted to Phys. Rev. Letters. Throughout this document, we investigate the importance of choices made in the analysis using Asimov sensitivities [2]. Although we will show in Section VII that Asimov sensitivities are flawed as a measure of true experimental sensitivity, their use is a convenient way to understand the impact of modifying the analysis.

---

\* Now at South Dakota School of Mines and Technology, Rapid City, South Dakota 57701, USA.

† Deceased.

‡ Now at Lancaster University, Lancaster, LA1 4YB, UK.

§ Now at CERN, CH-1211 Geneva 23, Switzerland.

In the 2016 MINOS sterile analysis [3], we directly compared the ratio of spectra in the Far (FD) and Near (ND) detectors (Far-over-Near ratio) in data and Monte Carlo (MC). This quantity, shown in Figure 1, had the advantage of being robust to systematic variations due to an explicit cancellation of systematic uncertainties that were correlated in the ND and FD, such as cross-section, beam, and reconstruction sources.

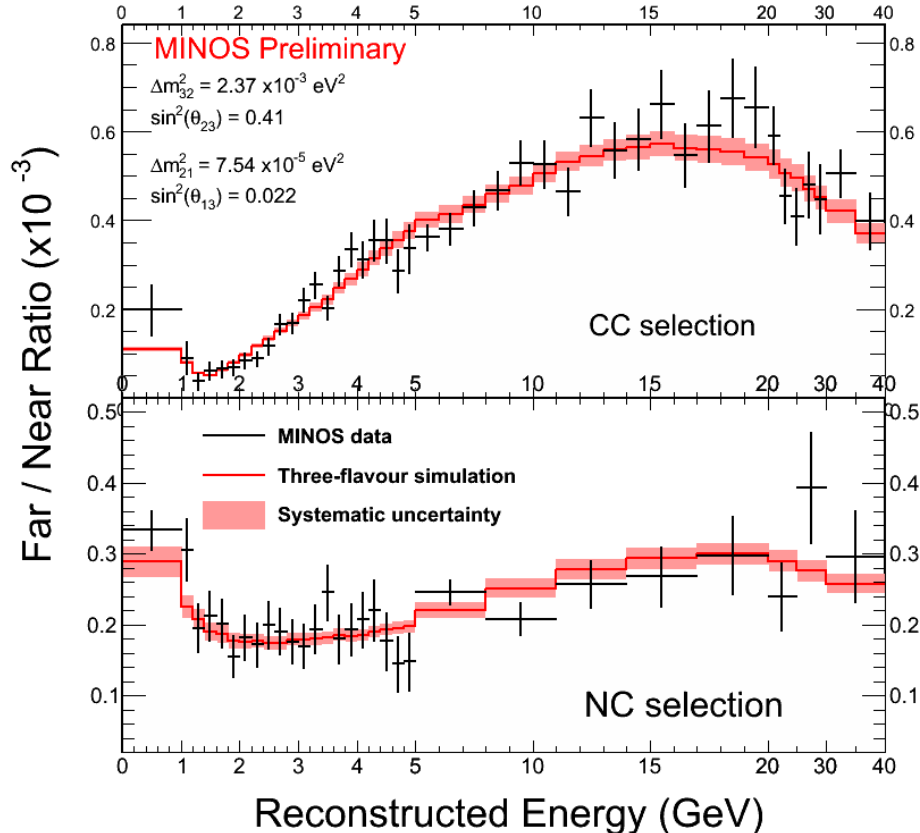

Figure 1. The Far-over-Near ratio using the full MINOS dataset for the  $\nu_\mu$ -CC selected sample (top) and the NC selected sample (bottom).

In the 2017 MINOS and MINOS+ sterile analysis [1], we have replaced our fit to the Far-over-Near ratio with a simultaneous two-detector fit using a covariance matrix describing the systematic and statistical uncertainties in both ND and FD, as well as the correlations between energy bins and between detectors arising from systematic uncertainties. This fit is called the two-detector fit.

We made this change due to two main shortcomings in the Far-over-Near ratio method. First, although the Far-over-Near ratio is robust against systematic uncertainties, the statistical uncertainty on the ratio is dominated by the statistical uncertainty of the FD, so the power of the ND is not fully realized. It reduces the sensitivity of the analysis to moderate to large  $\Delta m^2_{41}$  values where oscillations are primarily visible in the ND. Second, the Far-over-Near ratio reduces sensitivity to very large  $\Delta m^2_{41}$  scenarios where oscillations are primarily seen as normalization shifts in both detectors.

The two detector fit solves these shortcomings, but it creates its own challenges. Although the data/MC agreement for the Far-over-Near ratio is good, data/MC comparisons for the ND and FD spectra separately, seen in Figure 2 for  $\nu_\mu$  charged-current interactions (CC) and Figure 3 for neutral-current interactions (NC), show evidence of systematic variations. One major reason for this is the challenge of predicting the beam flux. In the 2016 analysis, we used an out-of-the-box FLUKA [4, 5] prediction for hadron production in the NuMI [6] beam target with systematic uncertainties on this prediction derived from a range of alternate flux models which were consistent with data collected by the NA49 hadron production experiment [7]. This was sufficient since hadron production uncertainties are dominated by normalization, so even large uncertainties left only small residual systematic uncertainties on the Far-over-Near ratio, on the order of 1%.

In the two-detector joint fit, we moved to using the PPFx package [8], an *a priori* flux prediction developed by the MINERvA experiment [9]. PPFx uses only hadron production experiment data and no NuMI neutrino data

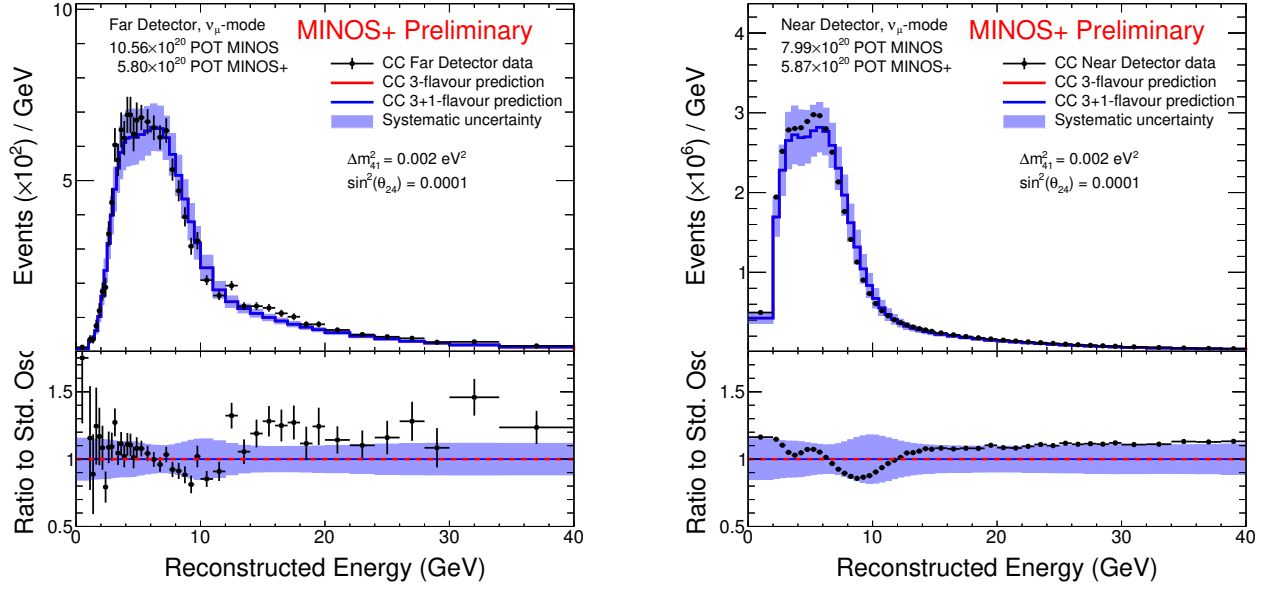

Figure 2. A comparison of data in the CC sample with the three-flavor prediction and the equivalent four-flavor MC prediction at  $\Delta m_{41}^2 = 2.33 \times 10^{-3} \text{ eV}^2$  and  $\theta_{24} = 0.011$  for the FD (left) and the ND (right). Similar systematic differences are present in the FD and ND.

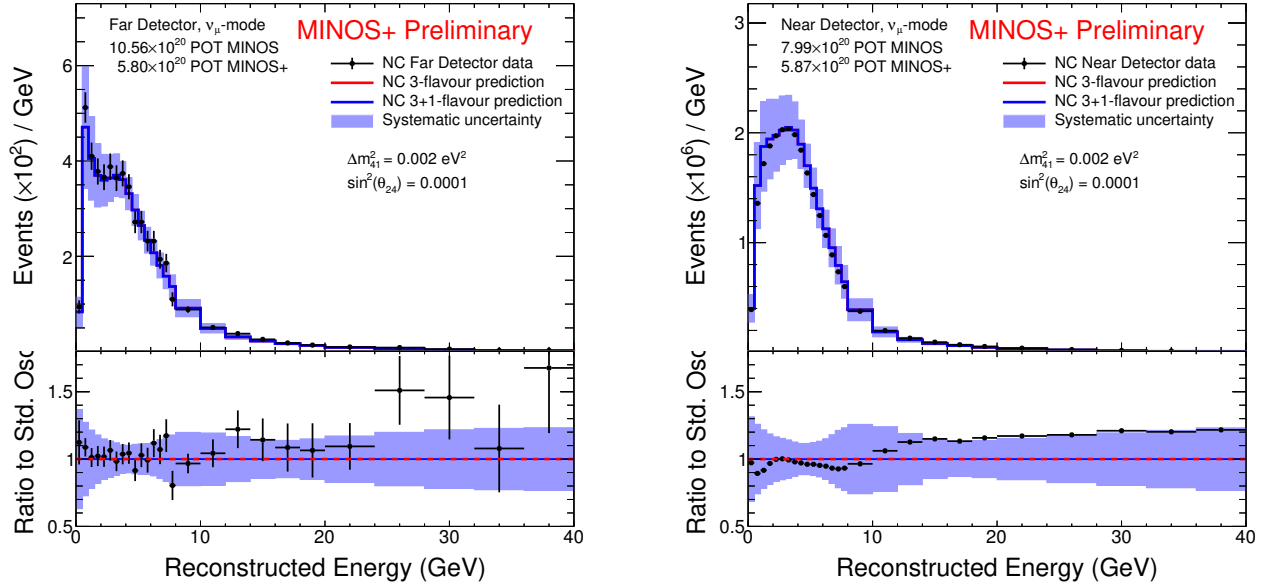

Figure 3. A comparison of data in the NC sample with the three-flavor prediction and the equivalent four-flavor MC prediction at  $\Delta m_{41}^2 = 2.33 \times 10^{-3} \text{ eV}^2$  and  $\theta_{24} = 0.011$  for the FD (left) and the ND (right).

itself to correct the out-of-the-box FLUKA flux prediction. This method provides both a central value that improves our data/MC agreement as well as a more robust estimate of systematic variation in hadron production. Using an *a priori* flux prediction is critical since an *a posteriori* method could potentially obscure a sterile neutrino signal by mis-attributing oscillation effects to corrections to the flux prediction derived from MINOS ND data. In fact, the differences between our data and MC, seen in Figures 2 and 3 are covered by the PPFX uncertainties.

Just as these data/MC disagreements canceled explicitly in the Far-over-Near ratio, they still cancel implicitly

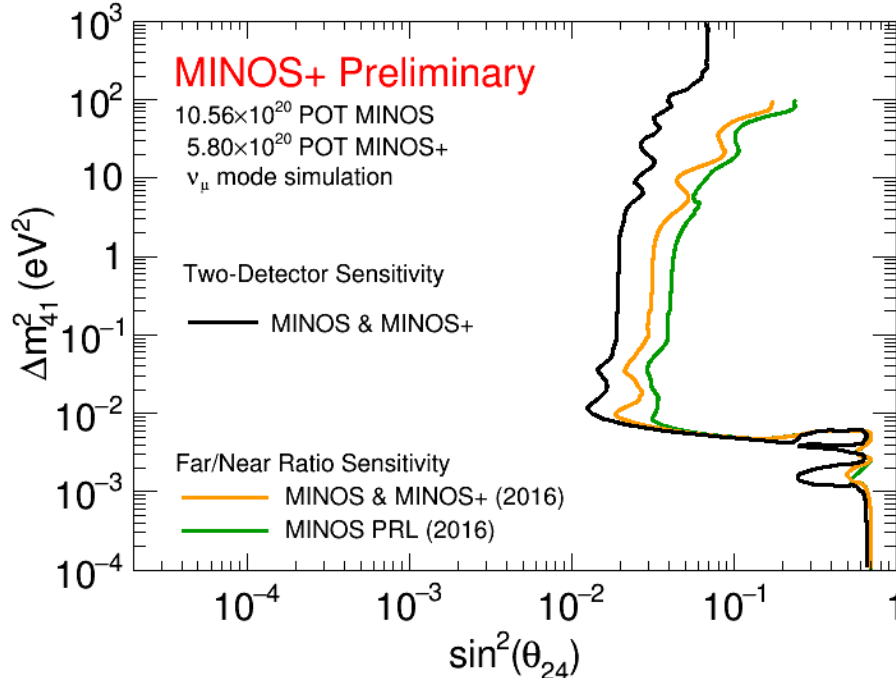

Figure 4. A comparison of sensitivities computed using the Far-over-Near ratio fit and the two-detector fit. Even without the addition of MINOS+ data, the two-detector fit produces more stringent limits for all  $\Delta m_{41}^2 > 0.01$  eV<sup>2</sup>, with particularly large improvements above 10 eV<sup>2</sup>.

through the off-diagonal terms in the covariance matrix, which contains correlations due to systematic variations allowed by the PPF method. Using a conditional multivariate Gaussian method, this implicit systematic cancellation can be made manifest. Figure 4 compares the Asimov sensitivities, that is, the sensitivity constructed using the median prediction, of the two-detector and Far-over-Near ratio methods in the  $(\Delta m_{41}^2, \sin^2 \theta_{24})$  plane.

In these supplemental materials, we provide extra details and context for the two-detector MINOS and MINOS+ 2017 sterile analysis beyond that present in our paper submitted to Physical Review Letters. In Section II, we will discuss the phenomenology of sterile neutrino oscillations at long baselines, where  $L/E \approx 500$  km/GeV and atmospheric oscillations are important, and explain how it differs from expectations at short baselines. In Section III, we describe in detail the most important sources of systematic uncertainty for this analysis. In Section IV, we will motivate why we chose to redesign our analysis around a two-detector fit instead of a Far-over-Near ratio. In Section V, we will detail the covariance matrix method for constructing the two detector fit, and we will describe how to use the conditional multivariate Gaussian distribution to impose the implicit systematic uncertainty cancellation. We will describe the contributions to the expected sensitivity from each detector, the relative power of the CC and NC samples, and the role of shape and normalization constraints. In Section VI, we analyze limiting cases where it is possible to predict the sensitivity to sterile neutrinos based on the sensitivity to atmospheric oscillations. In Section VII, we explain why the Asimov sensitivity [2] is a poor estimate of the median sensitivity. In Section VIII, we discuss assumptions made in the fit, and the impact of those assumptions on the final result. Finally, in Section IX, we will compare the expected sensitivity with the data limit and discuss features of the limit.

## II. PHENOMENOLOGY OF STERILE NEUTRINO OSCILLATIONS AT LONG BASELINES

Neutrino oscillations occur due to the mixing of mass and weak interaction flavor eigenstates described by the PMNS mixing matrix [10–12]. In the standard three-flavor scenario, the PMNS matrix is a unitary  $3 \times 3$  matrix parameterized as  $U = R_{23}R_{13}R_{12}$  [13], where  $R_{ij}$  is the rotation matrix for the angle  $\theta_{ij}$ . In this parameterization, if  $j - i \geq 2$ ,  $R_{ij}$  also contains a CP-violating phase,  $\delta_{ij}$ . The difference between the squares of the masses,  $\Delta m_{ji}^2$ , controls the frequency of the oscillations. The probability of a neutrino of energy  $E$  with initial flavor  $\alpha$  being detected with the flavor  $\beta$  after traveling a distance  $L$  is:

$$\begin{aligned}
P(\nu_\alpha \rightarrow \nu_\beta) = & \delta_{\alpha\beta} - 4 \sum_{i=1}^3 \sum_{j>i}^3 \text{Re} (U_{\alpha j}^* U_{\beta j} U_{\alpha i} U_{\beta i}^*) \sin^2 \Delta_{ji} \\
& + 2 \sum_{i=1}^3 \sum_{j>i}^3 \text{Im} (U_{\alpha j}^* U_{\beta j} U_{\alpha i} U_{\beta i}^*) \sin 2\Delta_{ji},
\end{aligned} \tag{1}$$

where  $\Delta_{ij} = \frac{\Delta m_{ij}^2 L}{4E}$ .

The 3+1 model is a simple extension of the three-flavor model of neutrino mixing with the addition of one new flavor state  $\nu_s$  and a new mass state  $\nu_4$ , extending the PMNS matrix to a  $4 \times 4$  unitary matrix. Under the parameterization  $U = R_{34}R_{24}R_{14}R_{23}R_{13}R_{12}$ , the extended matrix is written as:

$$U = \begin{bmatrix} U_{e1} & U_{e2} & e^{-i\delta_{13}} s_{13} c_{14} & e^{-\delta_{14}} s_{14} \\ U_{\mu 1} & U_{\mu 2} & -e^{-i(\delta_{13}-\delta_{14}+\delta_{24})} s_{13} s_{14} s_{24} + c_{13} s_{23} c_{24} & e^{-i\delta_{24}} c_{14} s_{24} \\ U_{\tau 1} & U_{\tau 2} & -e^{i\delta_{24}} c_{13} s_{23} s_{24} s_{34} + c_{13} c_{23} c_{34} - e^{-i(\delta_{13}-\delta_{14})} s_{13} s_{14} c_{24} s_{34} & c_{14} c_{24} s_{34} \\ U_{s1} & U_{s2} & -e^{i\delta_{24}} c_{13} s_{23} s_{24} c_{34} - c_{13} c_{23} s_{34} - e^{-i(\delta_{13}-\delta_{14})} s_{13} s_{14} c_{24} c_{34} & c_{14} c_{24} c_{34} \end{bmatrix}, \tag{2}$$

which introduces three new mixing angles,  $\theta_{14}$ ,  $\theta_{24}$ , and  $\theta_{34}$ , two new CP-violating phases,  $\delta_{14}$  and  $\delta_{24}$ , and one new linearly independent mass-splitting which we choose to be  $\Delta m_{41}^2$ .

We can simplify the oscillation probabilities in Equation 1 by neglecting  $\Delta_{21}$  and using unitarity to rewrite any terms containing  $U_{\alpha 1}$  or  $U_{\alpha 2}$ . The probability of  $\nu_\mu$  survival can be written:

$$\begin{aligned}
P(\nu_\mu \rightarrow \nu_\mu) \approx & 1 - 4 |U_{\mu 3}|^2 \left( 1 - |U_{\mu 3}|^2 - |U_{\mu 4}|^2 \right) \sin^2 \Delta_{31} \\
& - 4 |U_{\mu 3}|^2 |U_{\mu 4}|^2 \sin^2 \Delta_{43} - 4 |U_{\mu 4}|^2 \left( 1 - |U_{\mu 3}|^2 - |U_{\mu 4}|^2 \right) \sin^2 \Delta_{41}.
\end{aligned} \tag{3}$$

Since the three active flavors participate in the NC interaction at the same rate, the NC sample is unchanged by three-flavor oscillations. If a sterile neutrino exists, sterile neutrino appearance causes a depletion in the NC channel. Therefore, the NC survival probability is  $1 - P(\nu_\mu \rightarrow \nu_s)$ . Similar to Equation 3, this can be written:

$$\begin{aligned}
1 - P(\nu_\mu \rightarrow \nu_s) \approx & 1 - 4 |U_{\mu 3}|^2 |U_{s3}|^2 \sin^2 \Delta_{31} \\
& - 4 |U_{\mu 4}|^2 |U_{s4}|^2 \sin^2 \Delta_{41} \\
& - 4 \text{Re}(Z) (\sin^2 \Delta_{31} - \sin^2 \Delta_{43} + \sin^2 \Delta_{41}) \\
& - 2 \text{Im}(Z) (\sin 2\Delta_{31} + \sin 2\Delta_{43} - \sin 2\Delta_{41}),
\end{aligned} \tag{4}$$

where  $Z = U_{\mu 4}^* U_{s4} U_{\mu 3} U_{s3}^*$ .

The phenomenology of  $\nu_\mu$ -CC and NC disappearance driven by sterile neutrino oscillations is complicated at long baselines due to the interference of three-flavor oscillations and sterile oscillations, which does not occur at short baselines. To perform a two-detector analysis, effects at both short and long baselines must be understood. Figure 5 shows exact CC and NC oscillation probabilities as a function of  $L/E$  so that the effects at the ND and FD can be seen as part of a coherent picture.

We start by looking at the short-baseline approximation, valid only at the ND. For NC disappearance, the approximate oscillation probability is:

$$1 - P(\nu_\mu \rightarrow \nu_s) \approx 1 - \cos^4 \theta_{14} \cos^2 \theta_{34} \sin^2 2\theta_{24} \sin^2 \Delta_{41}, \tag{5}$$

where  $\Delta_{ji} = \frac{\Delta m_{ji}^2 L}{4E}$ . As seen in Figure 5, when  $\Delta m_{41}^2 < 0.05$ , oscillations are not visible in the ND. Starting at  $\Delta m_{41}^2 \sim 0.5 \text{ eV}^2$ , oscillations begin to be visible at low energies in the ND, and as  $\Delta m_{41}^2$  increases, the first oscillation maximum moves to higher energies. At sufficiently high  $\Delta m_{41}^2$  values, the entire ND sees rapid oscillations which can no longer be resolved and are seen as a constant normalization shift:

$$1 - P(\nu_\mu \rightarrow \nu_s) \approx 1 - \frac{1}{2} \cos^4 \theta_{14} \cos^2 \theta_{34} \sin^2 2\theta_{24}. \tag{6}$$

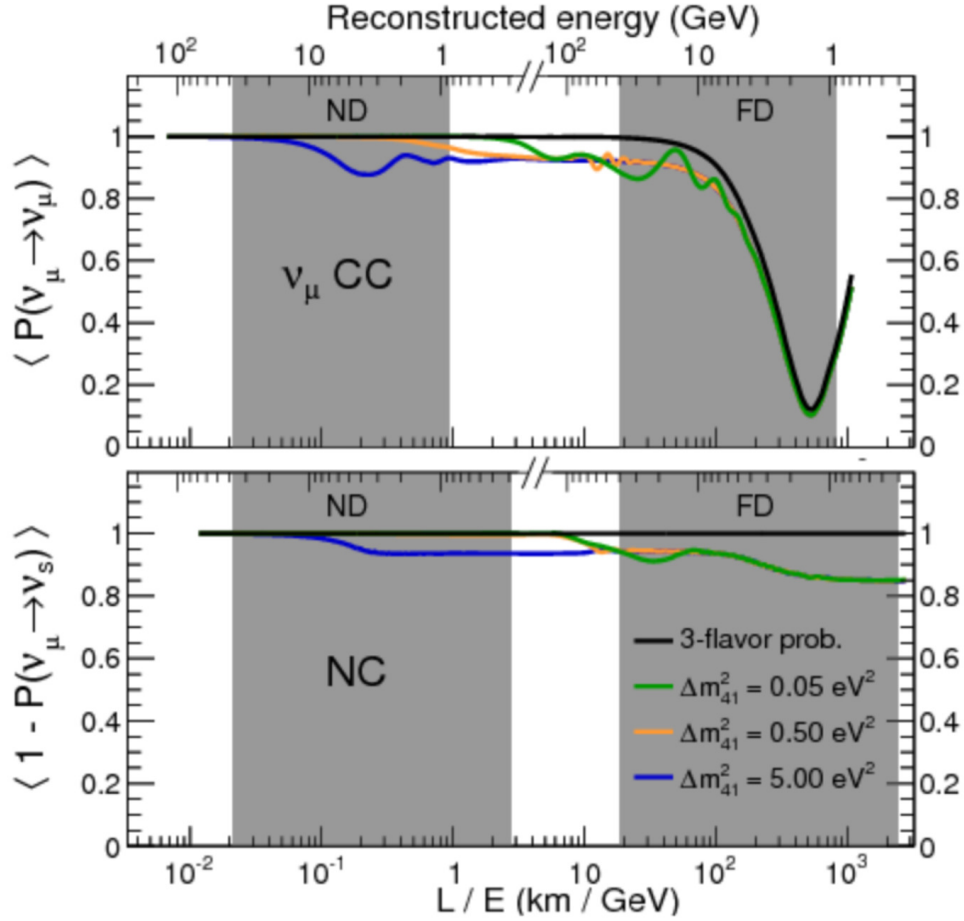

Figure 5. Muon neutrino oscillation probabilities as a function of  $L/E$ , where  $L$  is the distance traveled by the neutrinos, and  $E$  is the reconstructed neutrino energy, for three different values of  $\Delta m_{41}^2$ , with  $\theta_{14} = 0.15$ ,  $\theta_{24} = 0.2$ , and  $\theta_{34} = 0.5$ . All other oscillation parameters are taken from world averages. In both  $\nu_\mu$ -CC disappearance (top panel) and neutral current disappearance (bottom panel), there are minima at  $\sim 500$  km/GeV due to sterile neutrino oscillations at the atmospheric frequency.

For  $\nu_\mu$ -CC at the ND, the oscillation probability can be approximated as:

$$P(\nu_\mu \rightarrow \nu_\mu) \approx 1 - \sin^2 2\theta_{24} \sin^2 \Delta_{41}, \quad (7)$$

which behaves similarly to NC disappearance except it depends only on  $\theta_{24}$ , and in the rapid oscillation case, the normalization shift is given by  $(1/2) \sin^2 2\theta_{24}$ .

At long baselines, terms oscillating at the atmospheric frequency can no longer be neglected. Approximating the NC disappearance probability to first order in small mixing angles gives:

$$\begin{aligned} 1 - P(\nu_\mu \rightarrow \nu_s) \approx & 1 - \cos^4 \theta_{14} \cos^2 \theta_{34} \sin^2 2\theta_{24} \sin^2 \Delta_{41} \\ & - \sin^2 \theta_{34} \sin^2 2\theta_{23} \sin^2 \Delta_{31} \\ & + \frac{1}{2} \sin \delta_{24} \sin \theta_{24} \sin 2\theta_{23} \sin \Delta_{31}. \end{aligned} \quad (8)$$

In this, the first term is identical to the short-baseline approximation. The second and third terms both oscillate at the atmospheric frequency. If  $\theta_{34} > 0$ , the second term is non-zero, and if  $\sin \delta_{24}$  and  $\theta_{24}$  are non-zero, the third term will not be zero. In either case, this creates a dip at the FD regardless of the value of  $\Delta m_{41}^2$ . This is quite striking since NC disappearance is impossible in the standard three-flavor paradigm. It should also be noted that the third term is CP-odd since NC disappearance is effectively sterile neutrino appearance, so, in principle and parenthetically,  $\bar{\nu}$  data could add sensitivity.

For  $\nu_\mu$ -CC disappearance, we expand to second order in small mixing angles to get:

$$P(\nu_\mu \rightarrow \nu_\mu) \approx 1 - \sin^2 2\theta_{23} \cos 2\theta_{24} \sin^2 \Delta_{31} - \sin^2 2\theta_{24} \sin^2 \Delta_{41}. \quad (9)$$

By applying the double angle identity, we can rewrite this:

$$P(\nu_\mu \rightarrow \nu_\mu) \approx 1 - \sin^2 2\theta_{23} \sin^2 \Delta_{31} + 2 \sin^2 2\theta_{23} \sin^2 \theta_{24} \sin^2 \Delta_{31} - \sin^2 2\theta_{24} \sin^2 \Delta_{41}. \quad (10)$$

The first term is the standard approximation for three-flavor  $\nu_\mu$ -CC disappearance. The second term also oscillates as a function of  $\Delta m_{31}^2$ , the atmospheric frequency, but it is driven by sterile mixings. Even at large  $\Delta m_{41}^2$  values, this term does not enter into rapid oscillations. Figure 6 shows the ratio of four-flavor to three-flavor oscillations for  $\Delta m_{41}^2 = 1000 \text{ eV}^2$ . With such a large mass splitting, the ND is well inside the rapid oscillation regime; however, the FD still shows shape variations in addition to normalization changes due to the terms oscillating at the atmospheric frequency with a magnitude that scales with  $\sin^2 \theta_{24}$ . As seen in Figure 6, if we remove the expected  $\frac{1}{2} \sin^2 2\theta_{24}$  normalization shift from the ratio of four-flavor to three-flavor oscillations, we see shape effects that depend on the size of  $\theta_{24}$ .

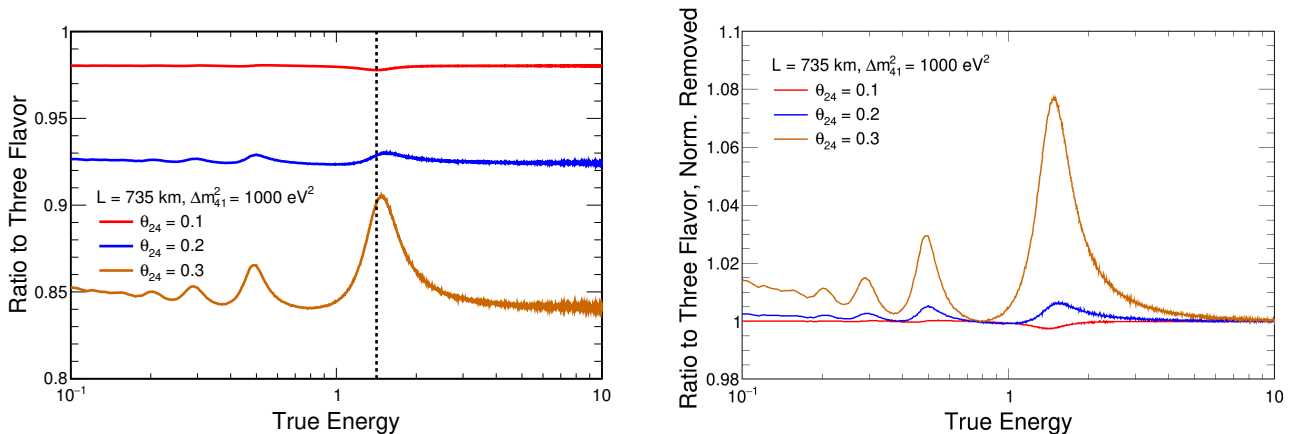

Figure 6. Left: The four-flavor/three-flavor ratio of  $\nu_\mu$  survival probabilities in the MINOS FD. Right: The four-flavor/three-flavor ratio of  $\nu_\mu$  survival probabilities in the MINOS FD divided by  $1 - \sin^2 2\theta_{24}$  to remove the normalization shift induced by rapid sterile oscillations. The four-flavor probabilities are computed at  $\Delta m_{41}^2 = 1000 \text{ eV}^2$ . At very large mass splittings, the effect of sterile neutrinos mostly creates a constant deficit relative to three-flavor oscillations; however, a term depending on the atmospheric frequency modifies the shape in a way that scales with  $\theta_{24}$ .

However, when considering  $\nu_\mu$  disappearance alone, we could define an effective atmospheric mixing angle to account for both sterile and standard oscillations by combining the first two terms in Equation 10:

$$\sin^2 2\theta_{23}^{\text{eff}} = \sin^2 2\theta_{23} \cos 2\theta_{24} \quad (11)$$

While it may seem that this implies that the depth of the atmospheric dip cannot tell us anything about the high  $\Delta m_{41}^2$  regime, it actually provides a constraint due to  $\theta_{23}^{\text{eff}}$  having been measured to be close to maximal. Due to the  $\cos 2\theta_{24}$  factor, a non-zero  $\theta_{24}$  can only drive  $\theta_{23}^{\text{eff}}$  away from maximal. As will be explained in Section VI, this, and related effects, drive our sensitivity to sterile neutrinos in several limiting cases.

### III. SYSTEMATIC UNCERTAINTIES

Many systematic uncertainties are considered for this analysis. Most are small, but a few, in particular cross-sections and energy scale, associated with the NC sample peak near 20%. However, most of these systematic uncertainties have

strong correlations between energy bins and between detectors that allow for a high degree of cancellation. Of these uncertainties, hadron production and our constraint on the overall cross-section scale are dominated by normalization uncertainties. We set a CC cross-section scale systematic of 3.5%. This can be justified by high energy cross-section studies. In particular, CCFR [14] probed the energy range 100 - 300 GeV and constrained the total cross-section to 3.0% with no indication of deviations from a linear dependence on energy [15]. In addition, CCFR had a short enough baseline ( $\sim 1.4$  km) to be able to see shape effects due to sterile neutrinos up to 1000 eV<sup>2</sup>. Due to their stringent limits [16], the constraint we use is valid. The NC cross-section scale uncertainty, at least at very high energies, should be directly related to the scale of CCs through the weak mixing angle; however, the extrapolation of this to lower energies is more uncertain due to potential differences in nuclear effects. To cover the disagreement between the ratio of the number of events with and without tracks at NOMAD [17] and MINOS, we increased the NC cross-section uncertainty to 5%.

### A. Hadron production

The three-flavor oscillations analyses in MINOS and MINOS+ searched for muon neutrino disappearance in the FD as predicted by the observation of the neutrino data spectrum in the ND. Standard three-flavor oscillations are negligible in the ND, so any discrepancy between data and simulation can be attributed to some form of mismodeling either in the detector or in the neutrino beam. A beam fit mechanism was employed in the three-flavor analyses in order to modify the MC simulation as a function of the underlying hadron phase space in such a manner that the data/MC agreement in the energy spectrum was improved. The systematic shifts determined by this beam fit can then be propagated through the simulation of the FD. In the 3+1 case, where oscillations can occur in the ND, performing a beam fit using ND data clearly has the undesirable effect of potentially attributing a data/MC disagreement due to oscillations to hadron production.

The most recent MINOS simulation of the neutrino flux in the NuMI beamline used the FLUKA simulation of the target and the FLUGG package [19] to propagate the resulting particles through a Geant4 simulation [20, 21] of the beamline geometry. The phase space of the parent hadrons produced in the target can be described using the kinematic parameters, transverse momentum ( $p_T$ ) and the longitudinal momentum ( $p_Z$ ). An initial fit using an empirical parameterization to the raw FLUKA simulation permits the determination of the effective functional form of the flux prediction in the  $p_Z$ - $p_T$  phase space, and the beam fit is then effectuated through a set of warping parameters which modify the parameterization as a function of  $p_Z$ . The result of this fit mechanism is the modification of the spectrum of neutrino events as a function of reconstructed neutrino energy based upon the underlying kinematic distribution of parent hadrons.

It has been shown in previous studies [18] that the ratio of  $\pi^+/K^+$  hadron production in the  $p_Z$ - $p_T$  phase space in the FLUKA simulation is well-tuned to data observations as can be observed in Figure 7. Using this information, identical adjustments are used for  $\pi^+$  and  $K^+$  parent hadrons sharing identical kinematic parameters.

For the present analysis, a new simulation of the flux from the NuMI beam, termed Package to Predict the Flux (PPFX) [8], was made available by the MINERvA experiment [9]. The PPFX framework derives an *a priori* flux prediction from hadron production experiments independent of the NuMI beam. While a full regeneration of the Monte Carlo simulation was computationally infeasible, the new flux prediction was incorporated into the spectra generated for this analysis via the reparameterization of PPFX using a variation on the beam fit mechanism described above.

The PPFX mechanism is only validated in the literature for neutrino energies  $< 20$  GeV, and the MINOS and MINOS+ spectra are predicted to be dominated by pion parents below this threshold as is shown in Figure 8. Therefore, the beam fit mechanism was applied to the PPFX flux prediction for neutrinos with pion parents in both the horn on and horn off beam configurations in order to determine the warping parameters describing the PPFX modifications to the raw FLUKA prediction. For reconstructed neutrino energies ranging from 20-40 GeV predicted contributions arising from kaon parents become significant. The application of these weights derived from the pion dominated phase space were found to be sufficient to improve the *a posteriori* agreement between data and simulation in this kaon dominated phase space. This joint fit method transforms the underlying neutrino flux into the de facto PPFX universes flux simulation for reconstructed energies  $< 20$  GeV while improving data/MC agreement for the energy range 20-40 GeV independent of all data used in the sterile neutrino search.

Given that the underlying flux simulation was improved for this analysis, the hadron production systematic uncertainty was recalculated using a method similar to the multi-universe construction employed by MINERvA. In the standard application of PPFX, an ensemble of many fluxes corresponding to various universes (i.e. sets of parameters defining possible states of nature) is produced using a set of correlated input parameters. In order to propagate the uncertainties associate with these parameters to the MINOS and MINOS+ flux prediction, each of the PPFX multi-universes was fit according to the method described above. The ensemble of fit results permits the construction

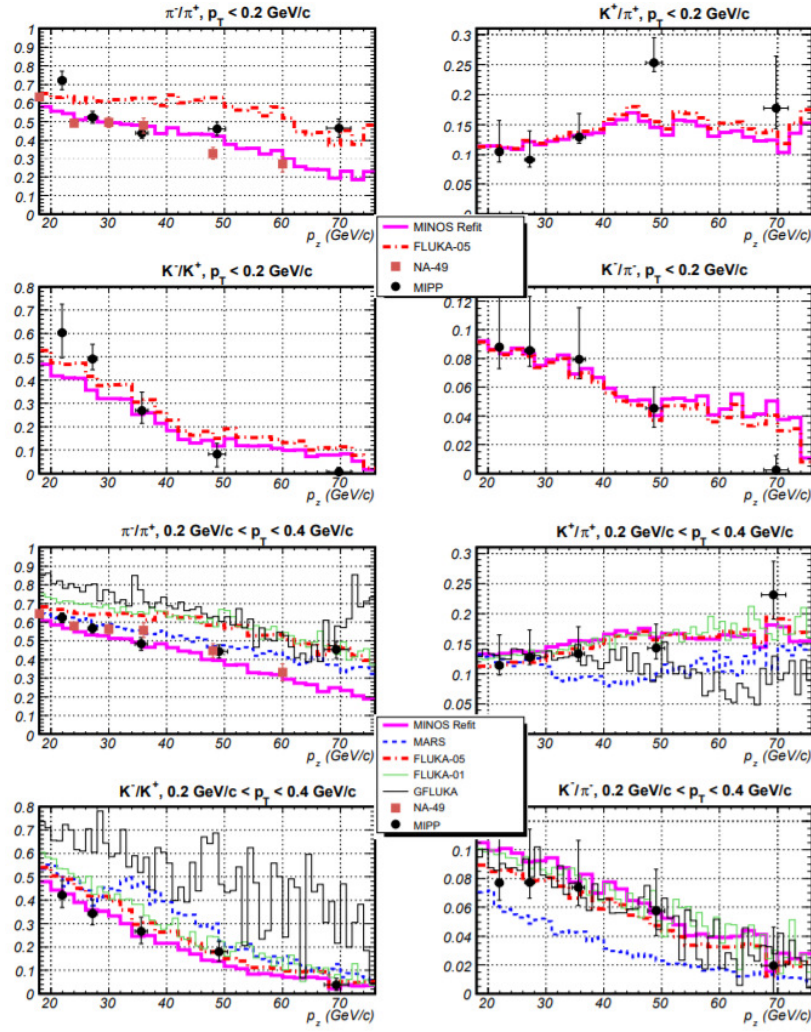

Figure 7. Comparison of the ratios of pions and kaons in data and FLUKA MC simulation in bins of transverse and longitudinal momentum. The right column shows the  $\pi^+/K^+$  ratio, which provides justification for the use of identical weights as a function of kinematic parameters. Taken from Ref. [18].

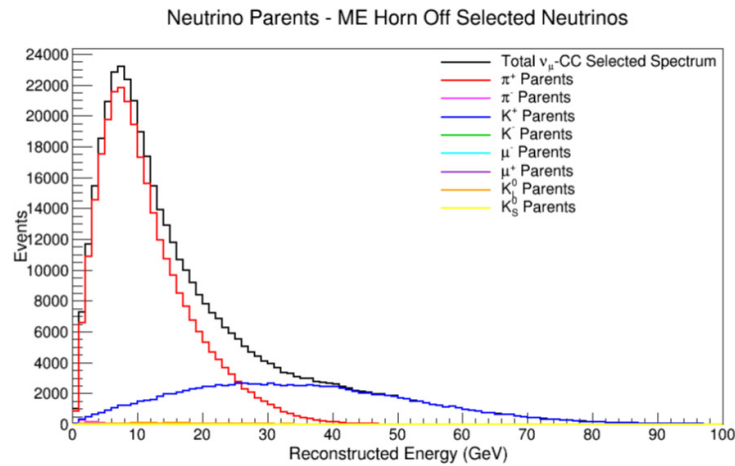

Figure 8. The simulated MC spectrum of reconstructed  $\nu_\mu$  CC events in the ND assuming no oscillations decomposed by parent hadron.

of a covariance matrix using the standard formalism

$$V_{ij} = \frac{1}{N} \sum_{\alpha}^N (n_{i\alpha} - \bar{n}_i)(n_{j\alpha} - \bar{n}_j) \quad (12)$$

where  $\alpha$  indexes the number,  $N$ , of universes simulated and  $i$  and  $j$  are indices of the  $i_{th}$  and  $j_{th}$  energy bins. The  $\bar{n}_i$  and  $\bar{n}_j$  are not necessarily equivalent to the central value weight in each bin and are instead the average over the simulated universes, which is computed from

$$\bar{n}_i = \frac{1}{N} \sum_{\alpha}^N n_{i\alpha} \quad (13)$$

In order to represent the spectral information encoded by the hadron production multi-universe method, the covariance matrix is decomposed into principal components. These principal components are presented for display purposes only and are not used in the fit. The first five principal components, which represent nearly the total variance of the hadron production covariance matrix, are plotted in Figure 9.

## B. Cross Sections

MINOS models neutrino cross sections using the NEUGEN [22] event generator, and cross-section uncertainties were assessed by changing NEUGEN parameters. The quasi-elastic cross section is modified by varying the axial mass  $M_A^{QE}$  by +35%/-15% where the upper bound was increased from +15% to account for 2p2h processes [23, 24] where neutrinos scatter off correlated nucleon pairs and the Random Phase Approximation (RPA) effect due to charge screening in the nucleus [25, 26]. The resonance cross section is modified by varying the axial mass  $M_A^{Res}$  +25%/-15%. In this case, the upper bound was increased only to account for the RPA effect.

The transition region between resonance and deep inelastic scattering is modeled by Koba-Nielsen-Olesen (KNO) [27] multiplicity parameters,  $r_{ijk}$ , where  $i = 1$  for CC interactions and 2 for NC interactions,  $j$  indicates whether a neutrino (antineutrino) interacted with a proton or neutron, and  $k$  indicates the multiplicity of the final state. We scale  $r_{1j(2,3)}$  by  $\pm$ ,  $r_{1(3,4)2}$  by  $\pm 0.2$ , and  $r_{2,j,(2,3)}$  by  $\pm 0.33$ . The high energy region is dominated by deep inelastic scattering where the uncertainty is treated as an overall scaling applied at all energies. For CC events, it is taken to be 3.5% and for NC events, it is taken to be 5%.

Antineutrinos are modeled using the same uncertainties as neutrinos, but we apply separate scale factors to account for uncertainties in the  $\sigma(\nu)/\sigma(\bar{\nu})$  ratio. For quasi-elastic and resonance events an extra 8% variation is applied, and an additional 4% variation is taken on the total cross section. The final cross-section systematic uncertainty bands are shown in Figure 10.

## C. Energy Scale

Energy scale uncertainties shown in Figure 11 are derived from a number of sources. First, muon track energy is varied within 2% if the track energy was computed using the track range and it is varied by 3% if the track energy was computed using the track curvature.

The hadronic shower energy scale consists of three parts. The relative hadronic energy scale is determined from the calibration procedure producing a 1.9% uncertainty for the ND and a 0.9% uncertainty for the FD. The absolute hadronic energy scale was determined through studies of the response of the CalDet test beam detector to pions [28]. This is taken to be 5%, correlated between the ND and FD.

Finally, an energy dependent uncertainty was assessed by modifying the model parameters of the INTRANUKE simulation [29] of intranuclear scattering of hadrons produced in neutrino interaction propagating out of the nuclear material [30]. The change in shower energy response was determined for variations of pion and nucleon cross sections and changes in the final state interaction and formation zone models. Adding the effect of varying 15 parameters in quadrature produced an exponentially falling systematic uncertainty as a function of shower energy with a maximum uncertainty of 3.5%. Since this is the result of the combination of several different uncertainties, the hadronic shower energy scale uncertainty is taken as fully uncorrelated both bin-by-bin and between detectors to be conservative.

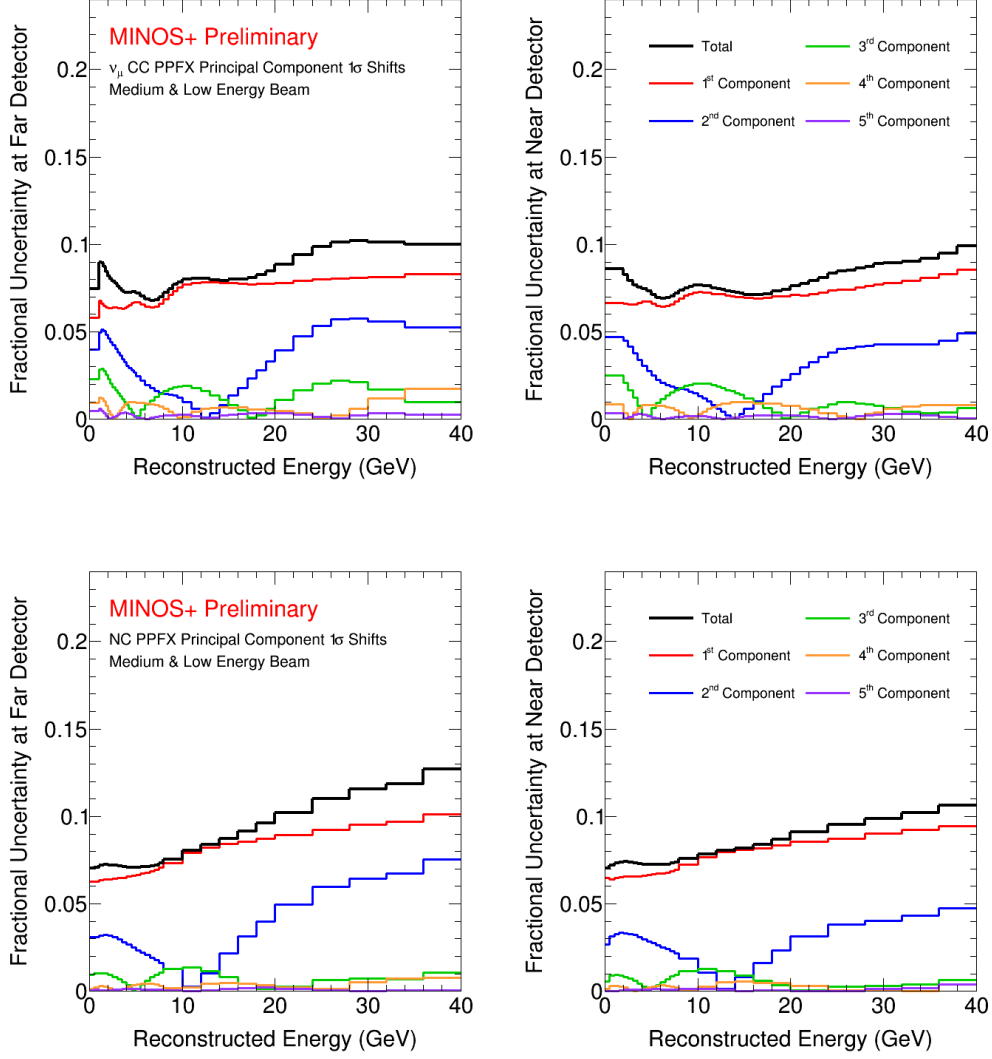

Figure 9. Hadron production uncertainties for CC (top), NC (bottom), FD (left), and ND (right). Hadron production uncertainties result from generating many alternate fluxes reweighted using the PPFX procedure with input parameters randomly varied within their uncertainty. To visualize the uncertainties, the resulting covariance matrix is decomposed into principal components representing the most important correlated sources of variation. The black curve represents the sum of all pictured uncertainties in quadrature.

#### D. Beam optics

The beam optics uncertainties estimate the uncertainty associated with systematic biases in the focusing apparatus of the NuMI beam [6]. Spectra of relative uncertainties for each of the beam optics categories are found in Figure 12 and 13. A total of seven sources of uncertainty are known to affect the focusing of the beam:

- Horn Current Miscalibration
- Horn Current Skin Depth
- Horn 1 Position Offset
- Target Position
- Material Error

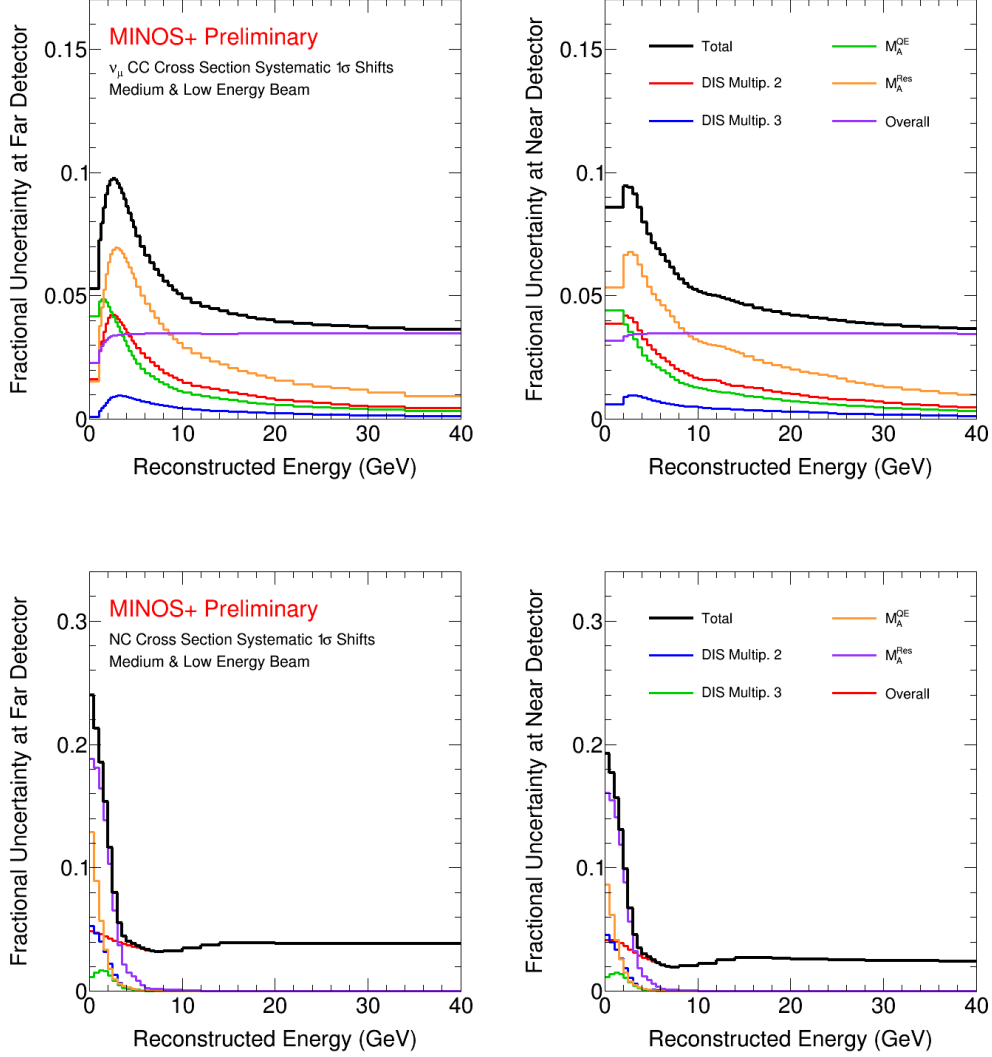

Figure 10. Cross-section uncertainties for CC (top), NC (bottom), FD (left), and ND (right). The overall cross-section scaling is effectively a normalization shift. This is constrained by high energy experiments like CCFR for the CC events. The NC cross-section scale uncertainty was determined by comparing rate of events with tracks to those without tracks at NOMAD and MINOS. Shape based uncertainties result from scaling  $M_A^{QE}$ ,  $M_A^{res}$ , and KNO scaling parameters. The black curve represents the sum of all pictured uncertainties in quadrature.

- Beam Position
- Beam Width

Due to variations in the electrical resistance of the focusing horns during the cycle of beam incidence, it is difficult to precisely determine the instantaneous current delivered to the focusing horns. The magnitude of the horn current has a direct effect on the ultimate position of the peak of the energy spectrum and is critical to an oscillations analysis. Miscalibration of the horn current represents the largest individual contribution to the focusing systematic uncertainty. In previous analyses, the uncertainty on the horn current was taken to be  $\pm 0.5\%$  in the delivered horn current where the nominal horn current is assumed to be 185 kA in the low-energy beam and 200 kA in the medium-energy beam. This was based on factory calibrations of current transformers used in the horn power supply, measurements of the horn current and resulting magnetic field taken on a test stand, and an in-situ calibration of the production power supply.

However, comparisons of data and simulation have shown a mismodeling of the peak of the neutrino energy distri-

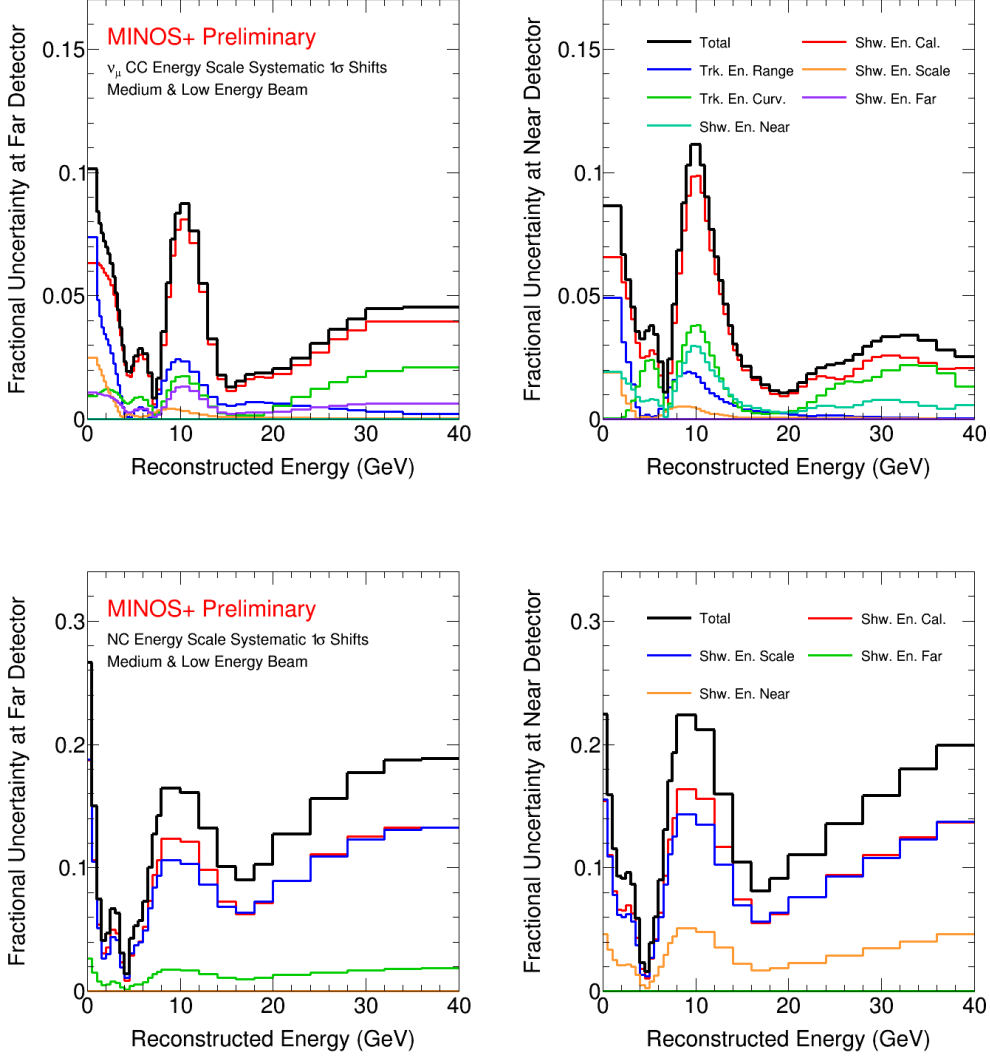

Figure 11. Energy scale systematic uncertainties for CC (top), NC (bottom), FD (left), and ND (right). This includes uncertainties on the calibration of the calorimetric response, the track energy scale by curvature or range, and the modeling of how much hadronic energy is produced by the neutrino interaction. The black curve represents the sum of all pictured uncertainties in quadrature.

bution. A study of data taken with the horn operating with a range of horn currents shows a consistent mismodeling of the peak of the neutrino energy distribution which can be explained by a constant 10 kA offset in the horn current in simulation relative to what is used in data. Since this effect is constant over a range of horn currents, and hence, a range of peak energies, this is not consistent with a sterile neutrino explanation. The two-detector fit shown in Section V is robust against a 10 kA correction to the nominal horn current, so instead of applying this correction, we have chosen to expand the miscalibration uncertainty from  $\pm 0.5\%$  to  $\pm 2.0\%$ .

If the focusing horns were ideal conductors, the entirety of the current delivered during a beam spill would pass along the outer surfaces. Since the horns are non-ideal, the skin depth  $\delta$  to which the current can penetrate the surface of the horns can be computed. Calculation of this skin depth indicates that it is in excess of the measured thickness of the horn material (2 mm for the inner conductor of horn 1, except in the neck region where it is 4.5 mm [6]) indicating that a model of uniform current distribution may be assumed. The uncertainty on this model choice is quantified by taking the relative difference between spectra modeled using  $\delta = 6$  mm (exponential current distribution) and the nominal infinite skin depth (uniform current distribution).

The modeling of the position and alignment of both the focusing horns and the production target is an additional

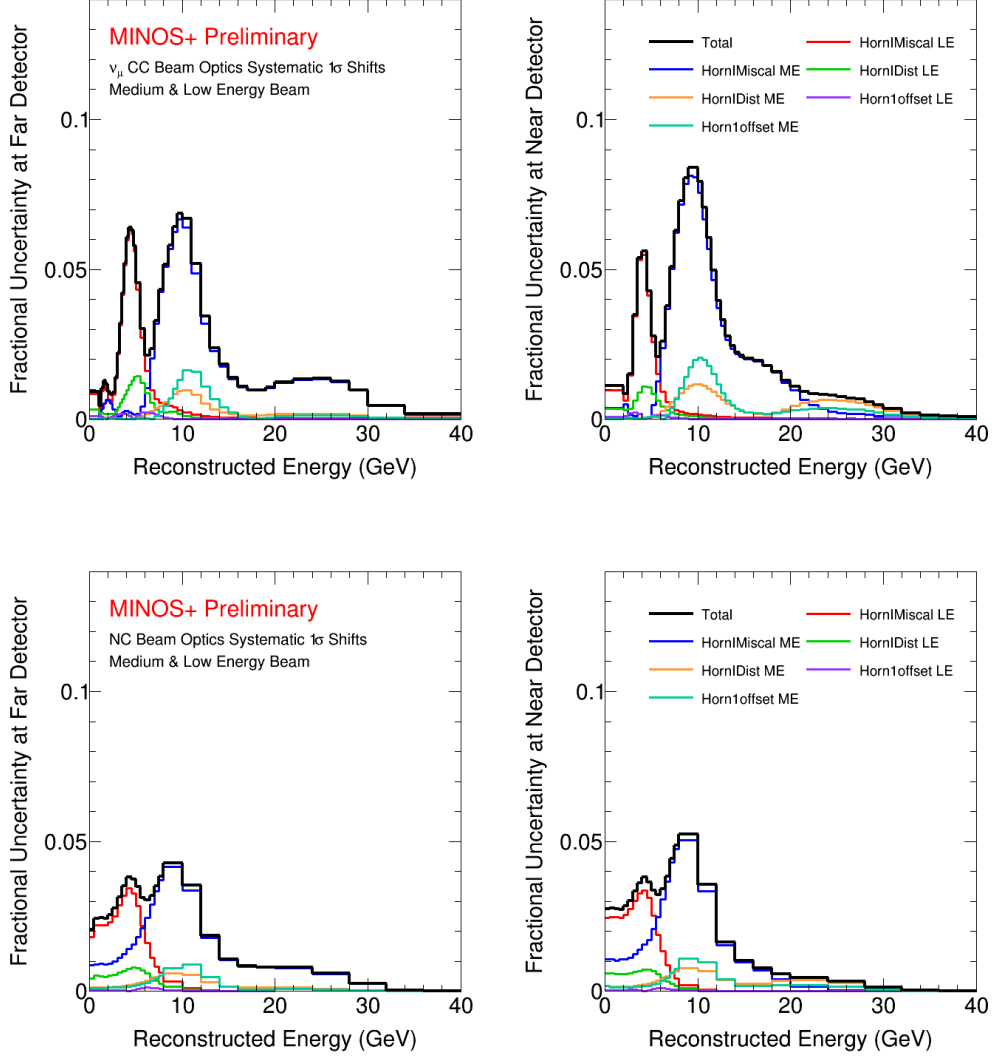

Figure 12. Beam optics systematic uncertainties for CC (top), NC (bottom), FD (left), and ND (right). This set includes a 2% variation in horn current and the effect of modeling the current distribution in the conductor as exponential or linear. The black curve represents the sum of all pictured uncertainties in quadrature.

important element in determining the position and shape of the predicted energy spectrum. The uncertainties for the horn and target positions were computed for offsets of 0.5 mm and 0.2 cm, respectively.

The final sources of uncertainty affecting the beam optics are related to the position and width of the beam spot on the target and focusing geometry. A variation in either of these parameters can lead to a significant number of protons missing the target. In order to minimize beam loss, only a single profile monitor is maintained in the beamline in order to determine the beam width, which leads to a significant increase in the uncertainty of the ultimate beam spot size. The relative uncertainties for the beam spot are computed for variations of  $\pm 0.5$  mm in the position and  $\pm 0.2$  mm in the width.

### E. Acceptance

The ND and FD are functionally equivalent to allow for the partial cancellation of systematic uncertainties, but the ND differs from FD in a few critical ways. First, the ND is much smaller than the FD, which necessitates the definition of a smaller fiducial volume in order to promote event containment. While both detectors are magnetized,

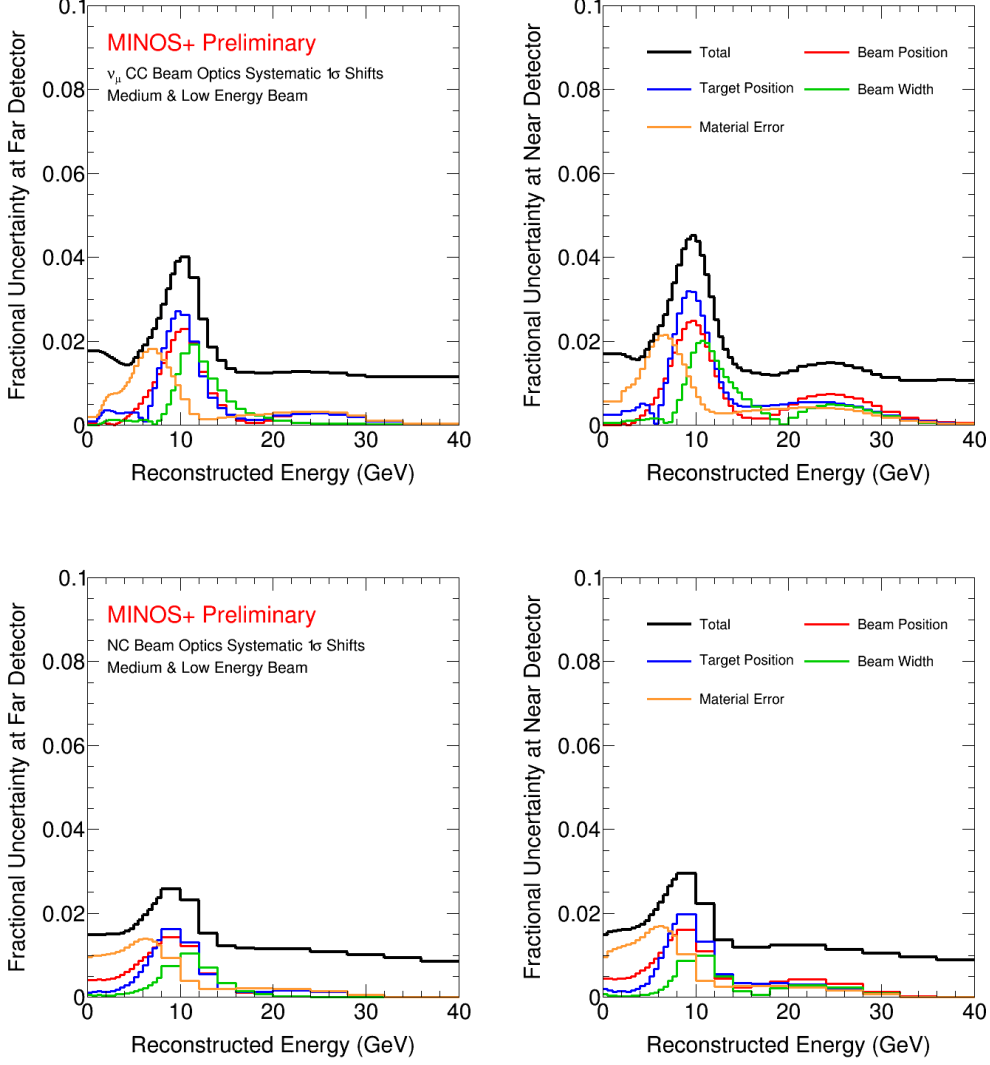

Figure 13. Beam optics systematic uncertainties for CC (top), NC (bottom), FD (left), and ND (right). This set includes variations in beam position, beam width, the measurement of POT, target position, and the amount of material in the beam line. The black curve represents the sum of all pictured uncertainties in quadrature.

the magnetic coil is offset from the beam center at the ND. The coil design and placement was designed to produce a similar magnetic field to the FD in the center of the detector, but the field is asymmetrical at the far ends of the fiducial volume. Finally, the downstream end of the ND is the spectrometer region, which contains four times as much steel as the calorimeter region.

Potential mismodeling is quantified by comparing data and MC using nominal selection criteria to data and MC using modified geometrical criteria using the formula:

$$\left( \frac{(\text{data}/\text{MC})_{\text{shifted}}}{(\text{data}/\text{MC})_{\text{nominal}}} - 1 \right) \left( \frac{\text{data}_{\text{shifted}}}{\text{data}_{\text{nominal}}} \right) \quad (14)$$

where the first term represents the fractional mismodeling of a subsample and the second term represents the proportion of that subsample in data. The full list of studied selection criteria modifications is:

- Selecting only events in either the left or right side of the fiducial volume
- Reducing the radius of the fiducial volume

- Allowing events with tracks which enter the coil hole region
- Removing events with tracks ending in the region around the join between the calorimeter and spectrometer
- Removing events with tracks exiting the back of the detector
- Removing events with tracks exiting the side of the detector

The resulting uncertainties are shown in Figure 14. The studied subsamples have no meaning beyond probing the level of mismodeling due to geometrical effects. That is, we do not expect a scenario where all events only occurred on one side of the fiducial volume. Instead, this is a conservative estimate of possible mismodeling. Since the shapes of the resulting uncertainties are not meaningful, we treat these uncertainties as being uncorrelated bin to bin.

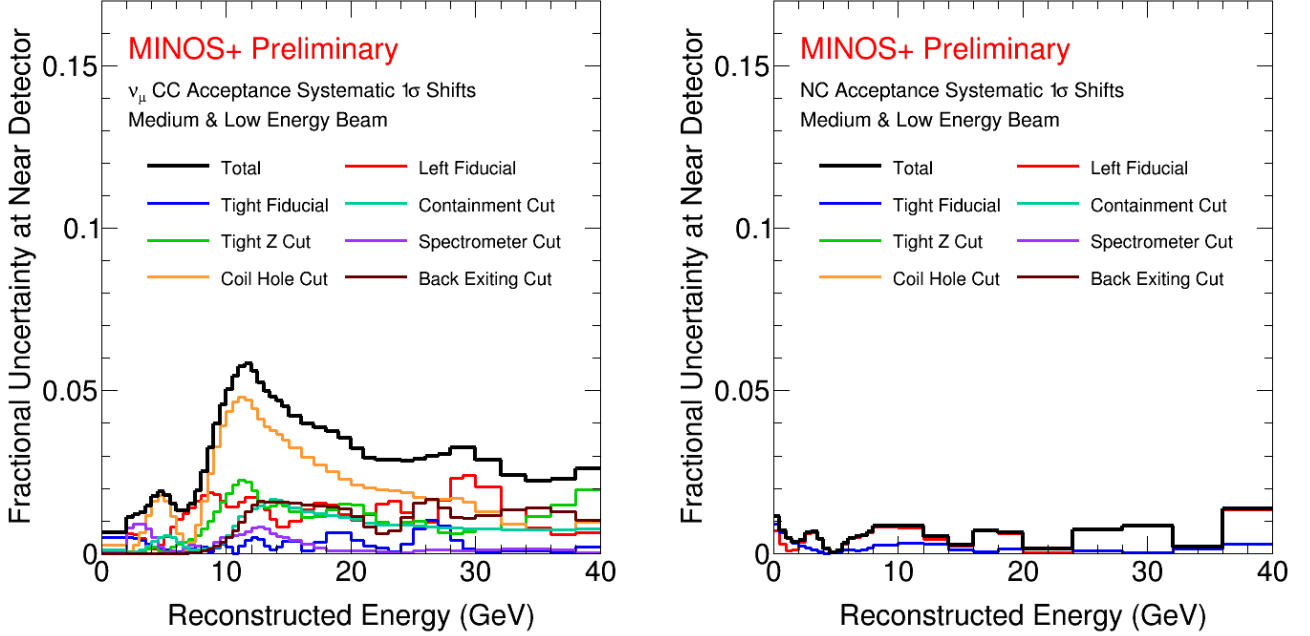

Figure 14. ND acceptance systematic uncertainties for CC (left) and NC (right). These uncertainties account for the different acceptance of the ND from the FD due to its small size and difference configuration by seeing how the data/MC ratio changes as cuts are modified. The black curve represents the sum of all pictured uncertainties in quadrature.

## F. Effective Normalization Uncertainty

All systematic uncertainties described above are a combination of shape and normalization effects. Since sterile neutrino oscillations can induce both shape modulations and overall normalization shifts, it is useful to be able to separate the systematic uncertainties into shape and normalization components.

An effective normalization uncertainty can be determined by sampling the  $\chi^2$  function, described in Section V, over a range of overall normalization shifts and determining the magnitude of the displacement which varies the  $\chi^2$  by one unit. This procedure is demonstrated in Figure 15 for the MINOS and MINOS+ two-detector fit, and the effective  $1\sigma$  normalization uncertainty is found to be 8.3% the CC sample and 9.6% for the NC sample. The normalization component is dominated by the hadron production systematic uncertainty.

The normalization component can also be extracted using a pseudo-experiment technique. In this technique, random fluctuations are drawn for each uncertainty and are applied to the Asimov sample. The resulting systematically shifted sample is then scaled to the same event count as the Asimov sample. The scale factor necessary to correctly normalize the fluctuated sample is the normalization component of the systematic shift for that sample. The standard deviation of the distribution of normalization shifts from a collection of fluctuated pseudo-experiments yields a 10.3% uncertainty for the CC sample and an 11.5% uncertainty for the NC sample.

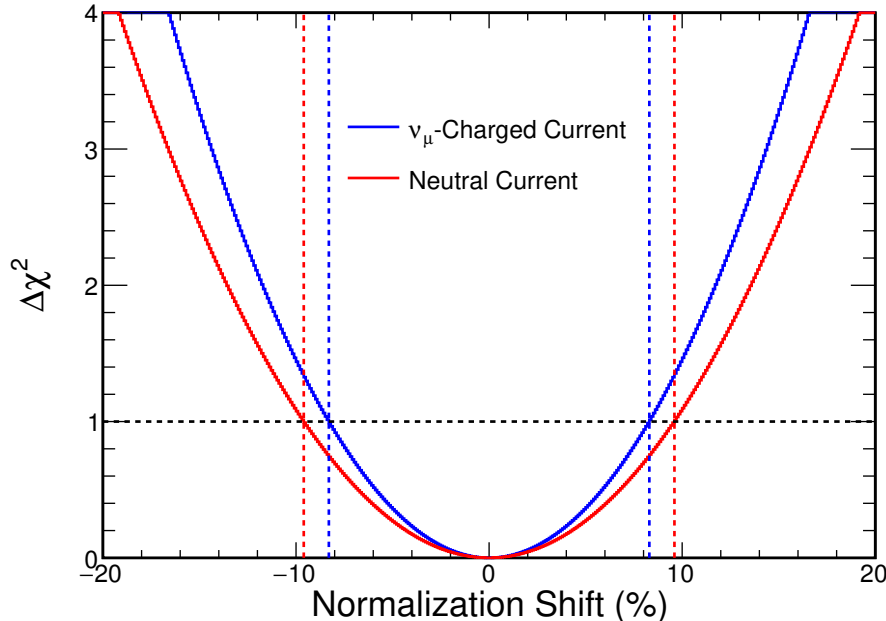

Figure 15. The  $\chi^2$  function for three-flavor fake data scaled by a normalization factor. This implies that the effective normalization systematic for the CC sample is 8.3% and for the NC sample is 9.6%.

#### IV. MOTIVATION FOR A TWO-DETECTOR FIT

The previous MINOS sterile analyses used a ratio fit method where the energy spectra of the MINOS FD was divided by the spectrum of the ND in order to search for modulations caused by the presence of sterile neutrinos, which was defined as the Far-over-Near ratio method in Section I. This method benefits from the straightforward reduction or potential cancellation of systematic uncertainties that have similar relative effects in both detectors such as cross sections on detector material and beam optics effects that are readily propagated forward from the ND to the FD. The ratio of spectra shifted by equivalent relative amounts clearly would not suffer from any reduction in sensitivity due to such a systematic effect. While the reduction of systematic effects is a benefit of the Far-over-Near method, this property also serves as a demonstration that such a method destroys information inherent in the measurements in the two detectors and can allow for the introduction of unwanted ambiguity and degeneracy. In fact, the lack of normalization information in the Far-over-Near method can make it less robust by permitting the fitting of shape effects which require unphysical normalization shifts.

For this present analysis, we have developed a two-detector fit method which simultaneously searches both detectors for the effects of sterile neutrinos. In this method, the systematic uncertainties are incorporated through the construction of a covariance matrix which includes the correlation of systematic uncertainties both within each detector and between the energy spectra of the two detectors, as will be discussed in detail in subsequent sections. The new method allows for the mitigation of the effects of systematic uncertainty without the destruction of information that occurs in a ratio method. The preservation of information from both detectors becomes critical to the maximal possible sensitivity of the search when considering the wide range of possible oscillations that may be observed.

In MINOS and MINOS+, oscillations arising from mixing with a sterile neutrino state may occur at baselines ranging from beyond the FD to before the ND. A selected example of the oscillation probabilities arising from various mass-splitting scales as a function of baseline divided by energy ( $L/E$ ) is shown in the left panel of Figure 16. Given that the three-flavor neutrino oscillation paradigm has been well-measured, further searches for oscillation phenomena depend on the observation of perturbations around the three-flavor probability. The modulations on the standard three-flavor probability are shown in the right panel of Figure 16 by taking the ratio of the 3+1 probability function with respect to three-flavor. Studying these probability curves permits several general conclusions. First, the first oscillation maximum shifts to smaller values of  $L/E$ , which corresponds to higher energy in each detector given the fixed baselines, as the mass-splitting scale becomes larger. Second, if a first oscillation maximum occurs in the FD, the ND spectrum remains largely unchanged, whereas if the first oscillation maximum occurs in the ND, the FD spectrum observes a net normalization offset due to smeared rapid oscillations. Third, if the oscillation maximum

occurs in the high energy regime of the ND, then both detectors observe a net normalization offset. Finally, if both detectors fall within the regime of rapid oscillations for the sterile mass-splitting, modifications are still present in the depth of the atmospheric oscillations. This case will be discussed further in Section VI.

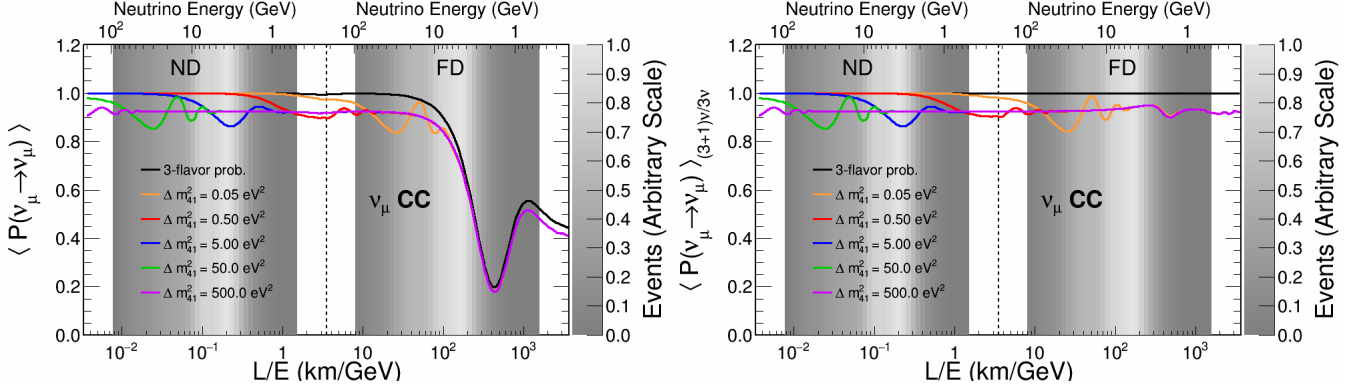

Figure 16. Left: Probability of  $\nu_\mu$  disappearance as a function of  $L/E$  with the position of the MINOS FD and ND indicated. Right: Ratio of the probabilities of  $\nu_\mu$  disappearance to the standard three-flavor oscillations probability. The shading of the detector regions in both plots indicates the relative magnitude of the predicted flux in arbitrary units. The upper axis gives the approximate neutrino energy corresponding to the  $L/E$  parameter in each detector.

A comparison of the Far-over-Near ratio and simultaneous two-detector fits methods is now possible taking into account the oscillation probabilities that may be observed. When oscillations are confined to the  $L/E$  regime corresponding to greater than or equal to the FD, there is no significant difference between methods as the ND serves only to establish the unoscillated spectrum, either as the denominator of a ratio or through cancellations within a covariance matrix. The power of the two-detector method is made apparent when considering oscillations occurring at  $L/E$  observable at the ND. In a Far-over-Near ratio fit, the ratio spectrum is always subject to the statistical uncertainties associated with the predicted event rate in the FD. For MINOS and MINOS+, the statistical uncertainties in the FD are on the order of 15% as compared to the  $< 0.1\%$  statistical uncertainty in the ND. Thus, even though modulations on the three-flavor paradigm in the ND can be observed in a Far-over-Near ratio fit, the sensitivity of the analysis is undermined by the statistical errors in the FD. In fact, it would be reasonable to expect a better measurement from a ND-only fit as compared to a Far-over-Near ratio fit when considering these short-baseline oscillations. A simultaneous two-detector fit permits a synergistic combination of the strengths of each detector without unduly penalizing the other.

A demonstration of the improvement in experimental sensitivity using a two-detector fit is illustrated in Figure 17. Consider the predicted reconstructed neutrino energy spectrum in both the FD and ND for the case where a sterile neutrino exists with  $\Delta m_{41}^2 = 80.0 \text{ eV}^2$  and  $\theta_{24} = 0.2$ . At this point in the parameter space, the Far-over-Near ratio contains only minimal oscillation behavior, which could not be disentangled from statistical or systematic uncertainties. However, when using a two-detector fit both the FD and ND observe a depletion in predicted event rate for the full range of reconstructed neutrino energies with a small oscillatory modulation in the high energy tail of the ND, making it possible to exclude this point in our final limit. Any oscillation signal with similar behavior becomes ambiguous in a Far-over-Near ratio fit but is readily detectable when utilizing the combined sensitivity of both detectors.

In order to quantify the improved sensitivity of the two-detector fit method, we compute the confidence interval in a sterile mixing parameter space as determined by fitting an Asimov experiment, which in the case of this analysis is the prediction for three-flavor neutrino oscillations. Contours showing the Asimov sensitivities for the Far-over-Near and simultaneous two-detector fit methods are presented in Figure 4. A comparison of the plotted contours demonstrates the increased sensitivity for all mass-splitting scales, though the most significant improvement is seen for  $\Delta m_{41}^2 > 10 \text{ eV}^2$ . The source of this dramatic increase in sensitivity is utilizing the full statistical power of the ND spectrum as was previously discussed. The contributions to the sensitivity from independent fits to the two detectors are compared to the simultaneous joint fit in Figure 18. The transition between the FD (red) and ND (blue) dominance of the sensitivity takes place at  $\Delta m_{41}^2 \sim 1 \text{ eV}^2$ . In the non-degenerate, FD dominated region,  $8 \times 10^{-3} \text{ eV}^2 < \Delta m_{41}^2 < 1 \text{ eV}^2$ , the two-detector sensitivity is more constraining than the FD-only sensitivity, even though the ND-only sensitivity does not constrain  $\sin^2 \theta_{24}$  in that region at all. This makes clear the value of the systematic uncertainty cancellation the ND provides. The simultaneous two-detector sterile neutrino search employs both a  $\nu_\mu$  CC sample fit jointly with an NC sample. The contributions to the experimental sensitivity for the individual and combined samples are also shown in Figure 18. The CC sample is the dominant source of sensitivity over the entire search range, though the NC events provide a cross-check on the observation of large mixing angles and a source

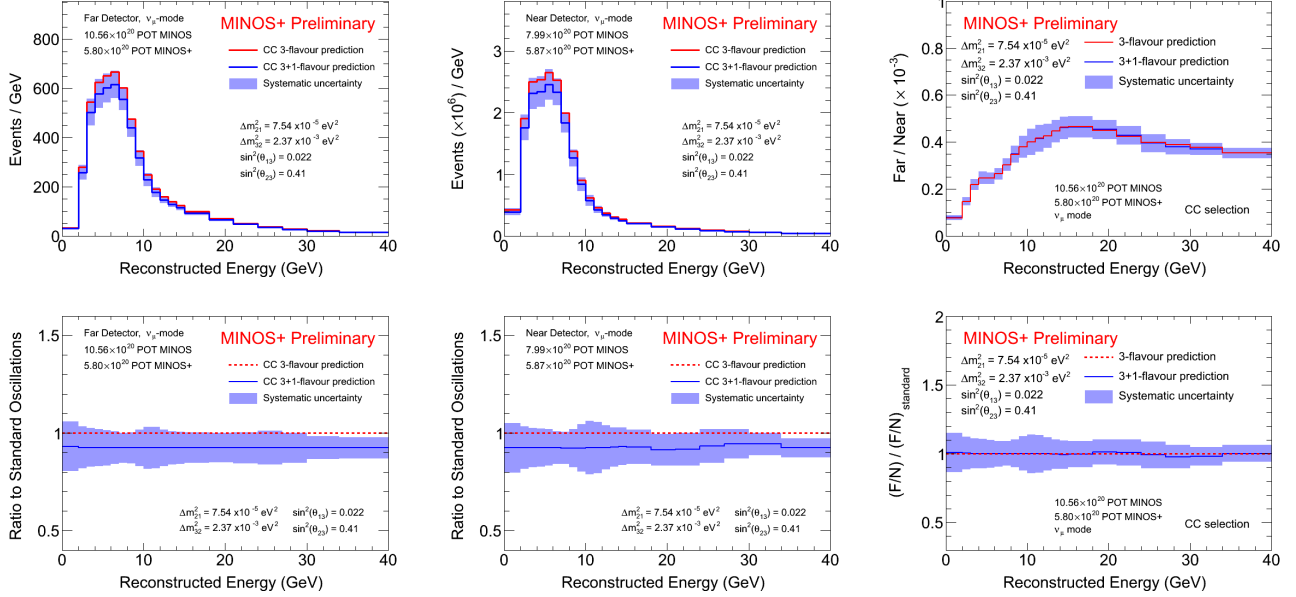

Figure 17. MC simulation of predicted reconstructed energy spectra and Far-over-Near ratio for three-flavor oscillations and a test point in parameter space where  $\theta_{24} = 0.2$  and  $\Delta m_{41}^2 = 80.0 \text{ eV}^2$ . This point is excluded in the final two-detector limit, but not be in a Far-over-Near analysis. Upper Left: Simulated FD reconstructed energy spectra. Lower Left: Ratio of simulated FD spectra with respect to three-flavor oscillations. Upper Center: Simulated ND reconstructed energy spectra. Lower Center: Ratio of simulated ND spectra with respect to three-flavor oscillations. Upper Right: Simulated Far-over-Near ratio reconstructed energy spectra. Lower Left: Double Far-over-Near ratios of simulated spectra with respect to three-flavor oscillations.

of disentanglement of degenerate parameters in the region where  $\Delta m_{41}^2 \approx \Delta m_{32}^2$ .

## V. MITIGATION OF CORRELATED SYSTEMATIC UNCERTAINTIES

In the 2016 MINOS sterile analysis [3], we fit the Far-over-Near ratio, which had the benefit of canceling many systematic uncertainties; however, the uncertainty of this ratio is dominated by the FD. In addition, the ratio eliminates the possibility of looking for sterile neutrinos through the interplay of normalization and shape effects. This degrades the sensitivity of the analysis at moderate  $\Delta m_{41}^2$  where oscillations are primarily seen as shape effects in the ND and at high  $\Delta m_{41}^2$  where oscillations are primarily seen as normalization effects at both detectors.

The joint two-detector fit using a covariance matrix encoding correlated uncertainties between energy bins and detectors corrects these problems, but it brings with it problems of its own. In particular, in a typical Poisson  $-\log \mathcal{L}$  fit, systematic uncertainties are accounted for through penalty terms which morph the fit function [31]. In such fits, post-fit agreement between data and MC is clear since the best-fit prediction includes both the effect of physics parameters and systematic uncertainties. In covariance matrix fits, the cancellation of correlated systematic uncertainties between the ND and FD is no longer easy to see since penalty terms are not used to modify the out-of-the-box prediction, and any error bars are strictly taken from the diagonal elements of the covariance matrix. This does not present a full picture of the post-fit agreement between data and MC. In this section, we will discuss how the covariance matrix fit is constructed and a method for visually accounting for correlated uncertainties.

### A. Covariance Matrix Fit

In this analysis we search simultaneously in both detectors for modulations on the standard oscillations due to sterile neutrinos by minimizing

$$\chi_{CC,NC}^2 = \sum_{i=1}^N \sum_{j=1}^N (x_i - \mu_i) [\mathbf{V}^{-1}]_{ij} (x_j - \mu_j) + \text{const.}, \quad (15)$$

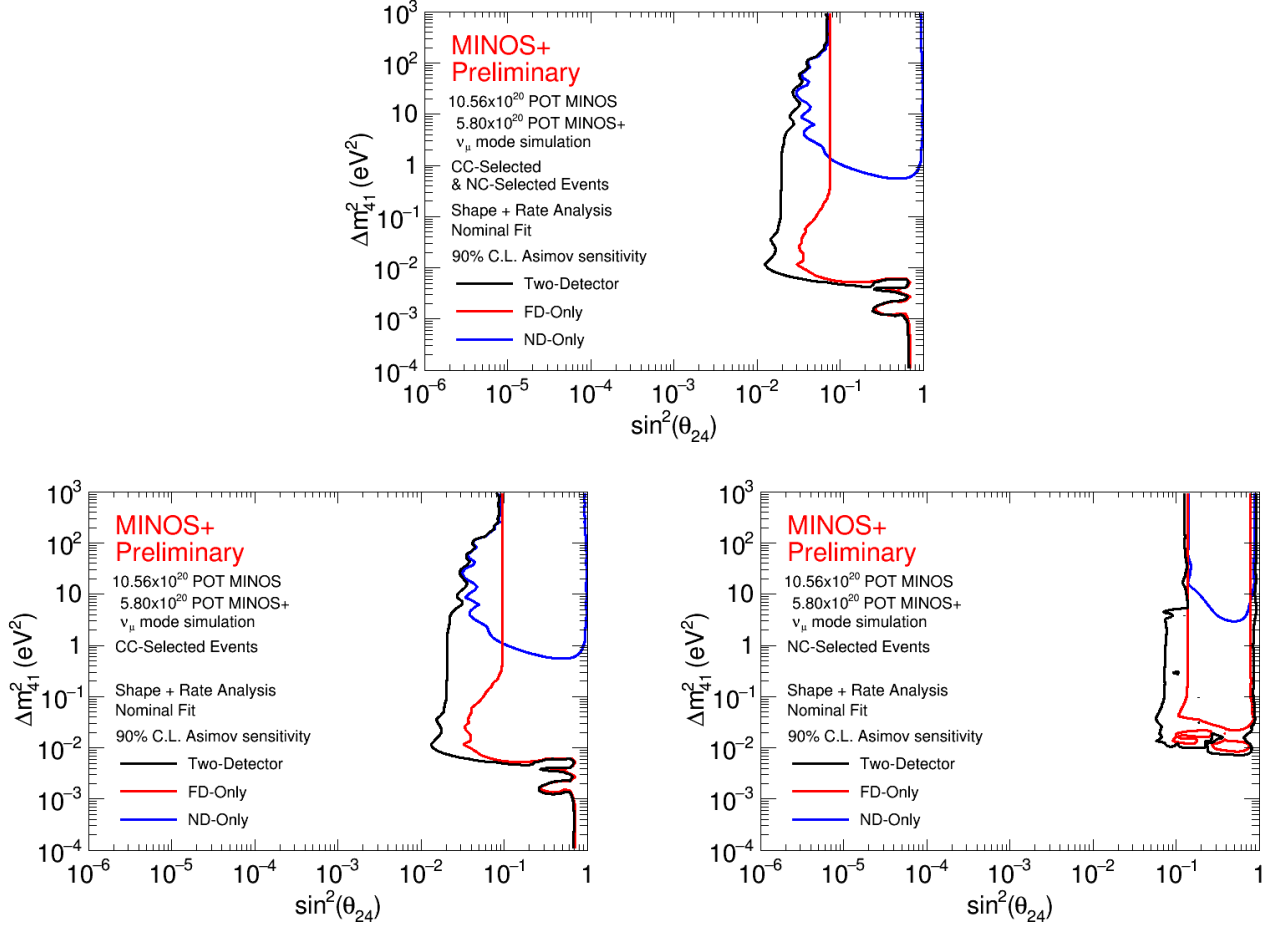

Figure 18. Asimov sensitivities for the two-detector fit method (black) compared with Asimov sensitivities considering either the Far (red) or Near (blue) Detector only. Top: Asimov sensitivities for the joint CC and NC-selected samples. Bottom left: Asimov sensitivities for only the CC-selected samples. Bottom right: Asimov sensitivities for only the NC-selected samples.

where the number of events observed in data and the MC prediction are denoted by  $x_i$  and  $\mu_i$ , respectively. The index  $i = 1, \dots, N$  labels the reconstructed energy bins from 0 to 40 GeV in each detector with  $N$  being the sum of ND and FD bins (91 bins in the CC sample, 54 bins in the NC sample). The predicted number of events  $\mu_i$  is varied using a MC simulation with exact forms of all oscillation probabilities in vacuum and includes all other experimental effects. The  $V^{-1}$  is defined as the inverse of the  $N \times N$  covariance matrix, which incorporates the sum of the statistical and systematic uncertainties.

The covariance matrix  $V$  is a sum of the component statistical and systematic uncertainty covariance matrices following the form:

$$V = V_{\text{stat}} + V_{\text{scale}} + V_{\text{had}} + V_{\text{xsec}} + V_{\text{bkgd}} + V_{\text{other}}, \quad (16)$$

where each term accounts for a particular source of uncertainty. The general structure of the covariance matrices is four quadrants corresponding to the FD covariance matrix, the ND covariance matrix, and cross-term matrices encoding the covariance between the detectors. The total covariance matrix has the form:

$$V = \begin{pmatrix} F_1 & 0 & \cdots & 0 \\ 0 & \ddots & & \\ & & F_k & \vdots \\ \vdots & & N_1 & \\ 0 & \cdots & 0 & N_m \end{pmatrix} + \sum_{i=1}^N V_i, \quad (17)$$

where the first matrix,  $V_{\text{stat}}$ , is diagonal and contains the statistical variances represented by  $F_i$ , the number of entries in the  $i$  FD bin, and  $N_j$ , the number of entries in the  $j$  ND bin. Here the index  $k$  indicates the number of bins in the FD prediction (47 bins for the CC sample, 27 bins for the NC sample) while the index  $m$  indicates the number of bins in the ND prediction (44 bins for the CC sample, 27 bins for the NC sample). The remaining  $V_i$  are covariance matrices encoding the correlated uncertainty from each source of systematic uncertainty. The covariance matrices used in the two-detector fit are shown in Figure 19. As opposed to the extrapolation technique, this method treats the ND and FD on equal footing to help disambiguate shape changes due to systematic uncertainties and neutrino oscillation signals.

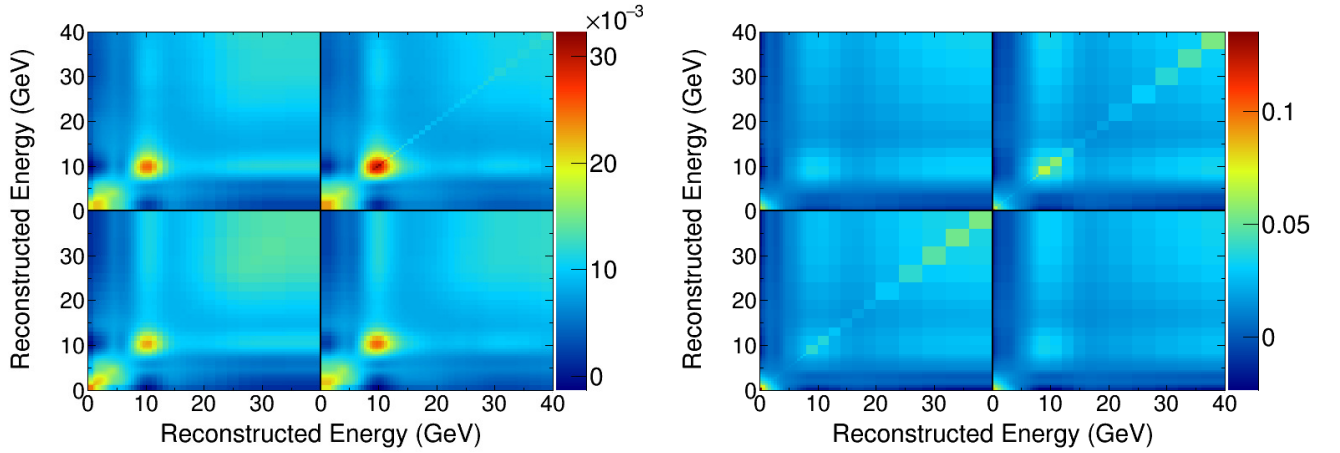

Figure 19. Left: The covariance matrix for the CC sample describing the systematic uncertainties of each bin and their correlations. Right: The covariance matrix for the NC sample.

### B. Systematic Cancellation in the Muon Neutrino CC Sample

The comparison of data and MC simulation in Figures 2 and 3, especially in the tail, raised concerns about potentially mismodeled systematic uncertainties. As described in Section V A, systematic uncertainties which were canceled through extrapolation or using the Far-over-Near ratio are now accounted for in a covariance matrix describing correlated uncertainties between bins and detectors. The covariance matrix treatment discounts the impact of the data/MC disagreements which have similarity with known systematic shapes in the resulting  $\chi^2$  value.

The power of the covariance matrix fit to minimize the impact of systematic uncertainties is similar to that achieved by the Near-to-Far extrapolation procedure. This can be visualized by applying a decorrelation procedure described in Appendix A to cancel correlated uncertainties and correct the prediction within the systematic band based on the observed data/MC agreement, though this procedure is never directly utilized in a covariance matrix fit. As shown in Figure 20, the decorrelation procedure makes apparent the significant systematic reduction achieved by the covariance matrix-based fit.

In addition to reducing the systematic uncertainty band, the decorrelation procedure also modifies the prediction. A comparison of the CC MC spectra with data after applying the decorrelation procedure can be seen in Figure 32. From this, we can see that the data/MC disagreement seen in Figures 2 is well described by systematic variations

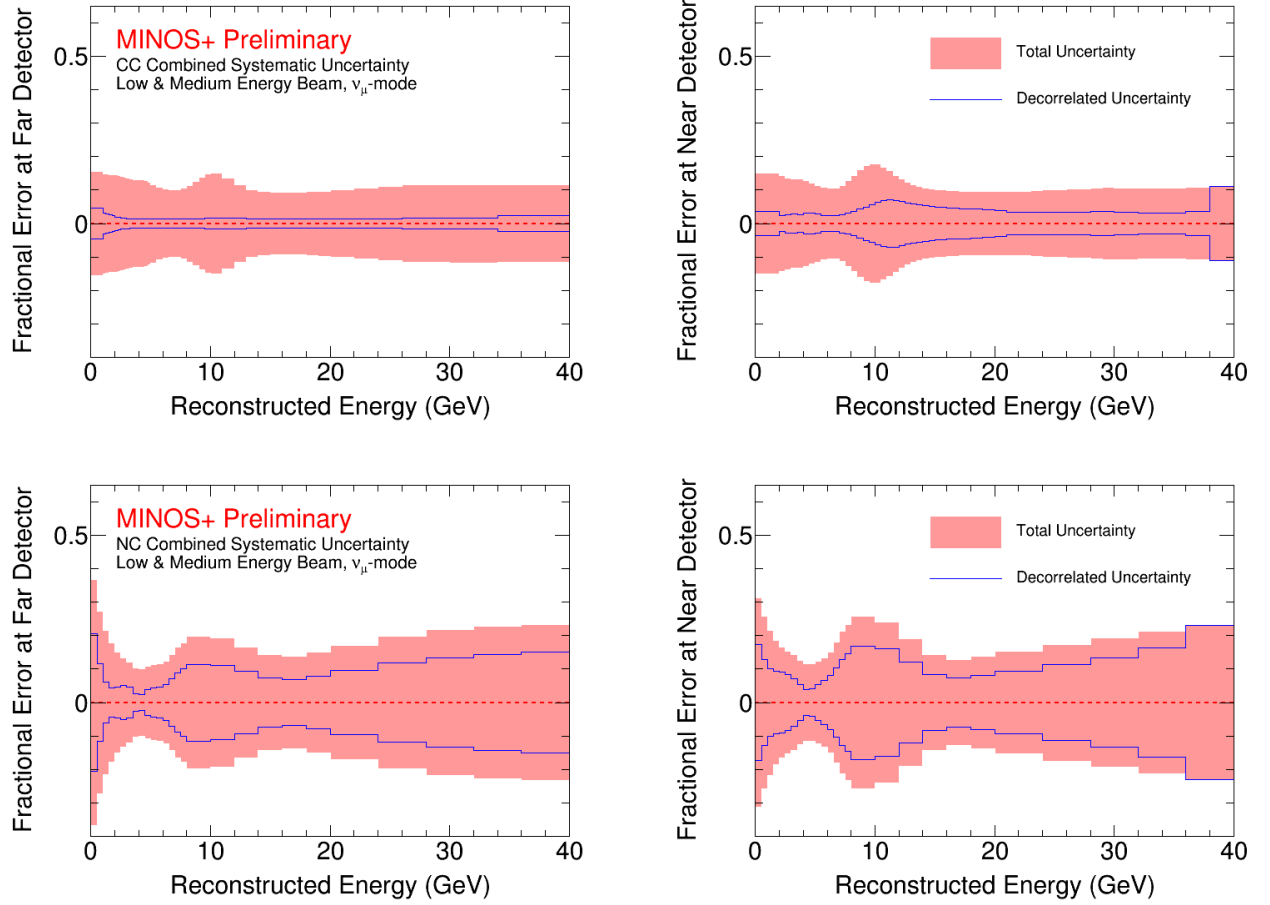

Figure 20. Top: The systematic error band (red), derived from the diagonal terms of the covariance matrix, for the CC sample in the FD (left) and ND (right). The blue band shows the reduced systematic uncertainty after decorrelating the uncertainties by correcting the nominal prediction given the observed value in the highest energy bin in the ND. Bottom: The systematic error band in the FD (left) and ND (right) derived from the diagonal elements of the covariance matrix (red) and after the decorrelation procedure (blue) for the NC sample.

embedded in the covariance matrix. The results of the decorrelation procedure on the NC sample can be seen in Figure 33.

### C. Shape vs. Normalization

Decorrelation of the covariance matrix (see Appendix A) and the resulting modifications both to the band of uncertainty and the spectral prediction makes manifest the complex interplay between the aspects of shape and normalization of the energy spectra. In this context, shape refers to an effect which morphs the energy spectrum without changing the total number of events, and normalization refers to an effect that changes the total number of events without morphing the spectrum.

To separate these effects, we developed a shape-only variant of our two-detector covariance matrix fit. To perform this fit, we construct shape-only covariance matrices using systematically fluctuated pseudo-experiments which have been normalized to the Asimov dataset. This is equivalent to subtracting a constant from each matrix element equal to the normalization uncertainty squared. In addition, an unconstrained normalization term is added to the fit. The resulting Asimov sensitivities for the two-detector fit, as well as an ND-only and FD-only fit, are shown in Figure 21 (left).

As will be discussed in detail in Section VI, the FD-only shape sensitivity at high  $\Delta m_{41}^2$  is due to the interference between sterile-driven oscillations and three-flavor atmospheric oscillations. Since three-flavor oscillations are neg-

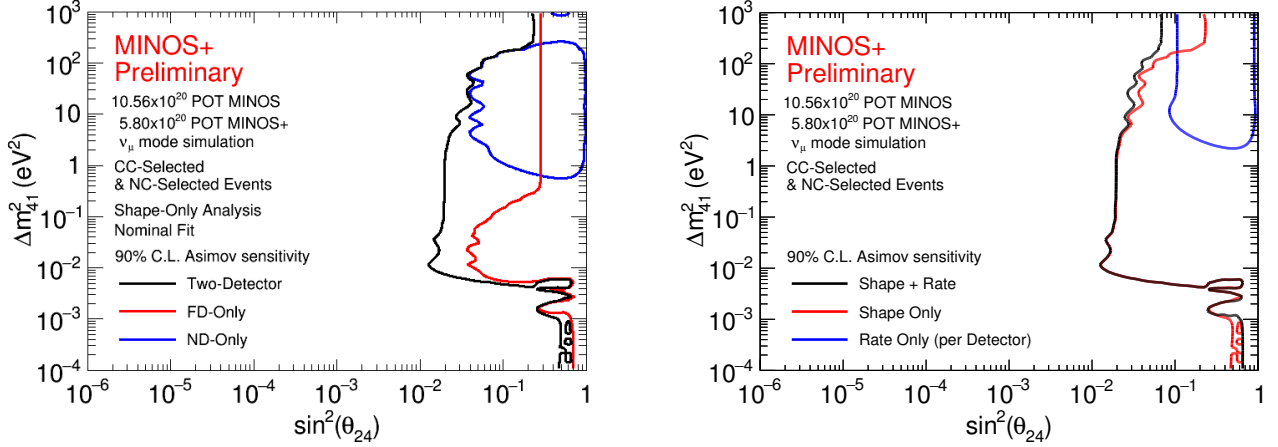

Figure 21. (Left) The shape-only 90% C.L. Asimov sensitivity as a function of  $\Delta m_{41}^2$  and  $\sin^2 \theta_{24}$ . The sensitivity at high and low  $\Delta m_{41}^2$  and well as at  $\Delta m_{41}^2 = 2\Delta m_{31}^2$  and  $\Delta m_{41}^2 = \Delta m_{31}^2$  directly depends on the three-flavor 90% C.L. sensitivity for  $\sin^2 2\theta_{23}$ . (Right) A comparison of our limit using our standard technique incorporating shape and normalization information (black), a shape-only fit (red), and a normalization-only fit (blue). The normalization-only fit treats each detector as a single bin with separate normalizations. Normalization information dominates for  $\Delta m_{41}^2 > 100$  eV<sup>2</sup> while shape information dominates at lower values.

ligible at the  $L/E$  of the ND, the ND-only fit has no shape sensitivity at high  $\Delta m_{41}^2$ . Critically, even though the ND-only fit is limited in sensitivity to the range  $0.5 \text{ eV}^2 < \Delta m_{41}^2 < 200 \text{ eV}^2$ , the two-detector fit is more sensitive than the FD-only fit almost everywhere. This is due to systematic uncertainty cancellation in the FD through the measurement in the ND.

A comparison of the shape-only Asimov sensitivity in Figure 21 (left) and the shape and rate Asimov sensitivity in Figure 18 shows that shape information dominates everywhere except in the region  $\Delta m_{41}^2 > 100 \text{ eV}^2$ . Using the short-baseline approximation shown in Equation 7, we can predict the expected Asimov sensitivity due to normalization alone at high  $\Delta m_{41}^2$ . The 90% C.L. sensitivity for counting experiment is defined by the region of parameter space for which the  $\chi^2$  is less than 2.71. Since the scale parameter in this regime is  $\frac{1}{2} \sin^2 2\theta_{24}$ , we can write:

$$\left( \frac{N - (1 - \frac{1}{2} \sin^2 2\theta_{24})N}{\sigma_N} \right)^2 < 2.71 \quad (18)$$

Rearranging, we find,

$$\frac{1}{2} \sin^2 2\theta_{24} < \sqrt{2.71} \frac{\sigma_N}{N} \quad (19)$$

where  $\frac{\sigma_N}{N}$  is the fractional uncertainty in the number of counts. Since the CC normalization, using the pseudo-experiment approach, is 10.3%, that implies that the normalization-only, CC-only 90% C.L. Asimov sensitivity should be  $\sin^2 \theta_{24} = 0.09$ . This is in good agreement with the CC-only Asimov sensitivity shown in Figure 18.

To test this, we perform a normalization-only fit where each detector and each sample is treated as a separate bin. In this case, the covariance matrix consists of four normalization uncertainties where the off-diagonal elements describe what fraction of the normalizations in the ND and FD are correlated. Figure 21 (right) compares the resulting normalization-only Asimov sensitivity with shape-only and shape + rate Asimov sensitivities. This confirms that normalization becomes dominant for  $\Delta m_{41}^2 > 100 \text{ eV}^2$ .

## VI. DEGENERACIES AND LIMITING CASES

In several special cases the sterile neutrino oscillation probability, and hence experimental sensitivities, become independent of  $\Delta m_{41}^2$ . These special cases arise from degeneracies between the sterile and three-flavor oscillation parameters and we consider the four cases below:

- $\Delta m_{41}^2 \rightarrow \infty$
- $\Delta m_{41}^2 = 2\Delta m_{31}^2$
- $\Delta m_{41}^2 = \Delta m_{31}^2$
- $\Delta m_{41}^2 \rightarrow 0$

Under these circumstances, a range of degenerate solutions become possible. An atmospheric degeneracy occurs if  $\theta_{23} = \theta_{34} = \frac{\pi}{2}$ , which eliminates NC disappearance, and atmospheric oscillations become driven by  $\theta_{24}$ . Assuming  $\theta_{13}$  and  $\theta_{14}$  are small,  $|U_{\mu 3}| \approx \cos^2 \theta_{24}$  and  $|U_{\mu 4}| \approx \sin^2 \theta_{24}$ . A quasi-degenerate solution where any apparent deviations from maximal mixing in the atmospheric oscillation maximum is due to sterile neutrinos occurs if  $\theta_{23} = \frac{\pi}{4}$ . In this case,  $|U_{\mu 3}| \approx \frac{1}{2} \cos^2 \theta_{24}$  and  $|U_{\mu 4}| \approx \sin^2 \theta_{24}$ . Finally, a reactor degeneracy occurs if  $\theta_{13} = \frac{\pi}{2}$ , which causes  $\theta_{14}$  to take over the role of  $\theta_{13}$  as measured by reactor experiments. In this case,  $|U_{\mu 3}| \approx 0$  and  $|U_{\mu 4}| \approx \sin^2 \theta_{24}$ . Using these cases, we can analytically predict the shape-only, 90% C.L. Asimov sensitivity, shown in Figure 21 (left), using only the three-flavor 90% C.L. sensitivity produced with the sterile analysis framework. From Figure 22, we see that  $\sin^2 2\theta_{23} > 0.89$  and  $0.35 < \sin^2 \theta_{23} < 0.66$  at 90% C.L.. We will next analyze how the full oscillation probability from Equation 3 simplifies in each limiting case.

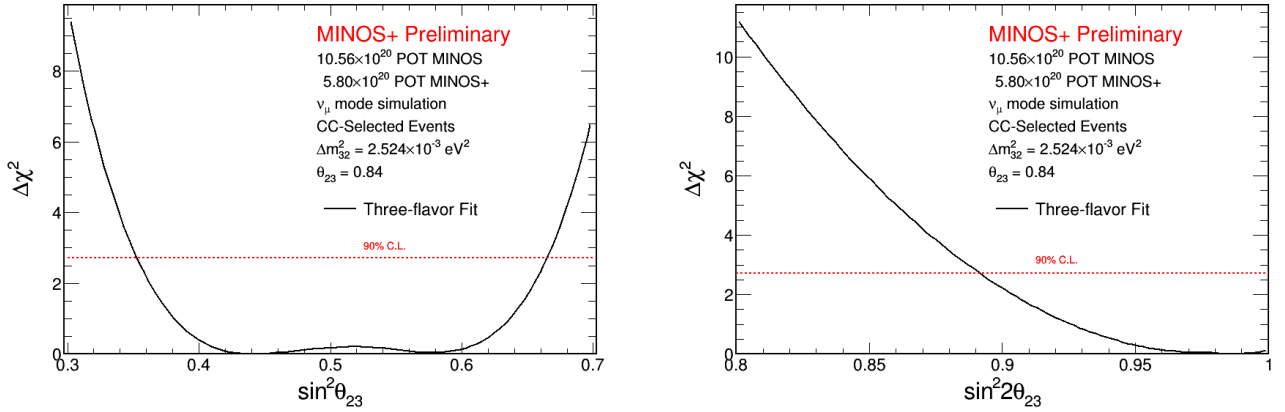

Figure 22. Left:  $\Delta\chi^2$  as a function of  $\sin^2 \theta_{23}$ . Right:  $\Delta\chi^2$  as a function of  $\sin^2 2\theta_{23}$ . In both cases, the CC-selected simulated sample was fit using the sterile neutrino analysis framework with  $\theta_{14}$ ,  $\theta_{24}$ , and  $\theta_{34}$  fixed to zero, and only  $\theta_{23}$  was allowed to vary. At 90% C.L., the resulting expected Asimov sensitivities are  $\sin^2 2\theta_{23} > 0.89$  and  $0.35 < \sin^2 \theta_{23} < 0.66$ .

#### A. $\Delta m_{41}^2 \rightarrow \infty$

When  $\Delta m_{41}^2 \rightarrow \infty$ ,  $\sin^2 \Delta_{43} = \sin^2 \Delta_{41} = \frac{1}{2}$  due to the finite resolution of the MINOS detectors. On Figure 21, this corresponds to the region  $\Delta m_{41}^2 > 100 \text{ eV}^2$ . This simplifies Equation 3 to:

$$P(\nu_\mu \rightarrow \nu_\mu) \approx 1 - 4|U_{\mu 3}|^2 \left(1 - |U_{\mu 3}|^2 - |U_{\mu 4}|^2\right) \sin^2 \Delta_{31} - \frac{1}{2}|U_{\mu 4}|^2 \left(1 - |U_{\mu 4}|^2\right). \quad (20)$$

In the atmospheric degenerate case, this produces a non-oscillatory solution, but in the quasi-degenerate case, this yields:

$$P(\nu_\mu \rightarrow \nu_\mu) \approx 1 - \cos^4 \theta_{24} \sin^2 \Delta_{31} - \frac{1}{2} \sin^2 2\theta_{24}. \quad (21)$$

where the  $\Delta_{31}$  term contains shape information, and the term with no  $L/E$  dependence controls the overall normalization. In the full shape + rate fit, the sensitivity in this region is driven by the constant term. However, a shape-only fit is only sensitive to the depth of the atmospheric dip relative to the asymptotic behavior controlled by the normalization term, so we consider the oscillation probability divided by the overall normalization:

$$\frac{P(\nu_\mu \rightarrow \nu_\mu)}{1 - \frac{1}{2} \sin^2 2\theta_{24}} \approx 1 - \frac{\cos^4 \theta_{24}}{1 - \frac{1}{2} \sin^2 2\theta_{24}} \sin^2 \Delta_{31}, \quad (22)$$

which implies that

$$\sin^2 2\theta_{23}^{\text{eff}} = \frac{\sin^4 \theta_{24} - 2 \sin^2 \theta_{24} + 1}{2 \sin^2 \theta_{24} - 2 \sin_{24}^2 + 1}, \quad (23)$$

which can be solved to show at 90% C.L.  $\sin^2 \theta_{24} > 0.26$  is excluded.

$$\mathbf{B.} \quad \Delta m_{41}^2 = 2\Delta m_{31}^2$$

When  $\Delta m_{41}^2 = 2\Delta m_{31}^2$ ,  $\Delta m_{43}^2 = \Delta m_{31}^2$ . On Figure 21, this corresponds to the region  $\Delta m_{41}^2 \approx 5 \times 10^{-3} \text{ eV}^2$ . This simplifies Equation 3 to:

$$\begin{aligned} P(\nu_\mu \rightarrow \nu_\mu) \approx & 1 - 4 \left( |U_{\mu 3}|^2 - |U_{\mu 4}|^2 \right) \sin^2 \Delta_{31} \\ & - 4 |U_{\mu 4}|^2 \left( 1 - |U_{\mu 3}|^2 - |U_{\mu 4}|^2 \right) \sin^2 2\Delta_{31}. \end{aligned} \quad (24)$$

The  $\sin^2 2\Delta_{31}$  term breaks the degeneracy unless  $\theta_{23} = \frac{\pi}{2}$ . The probability then becomes

$$P(\nu_\mu \rightarrow \nu_\mu) \approx 1 - 4 |U_{\mu 3}|^2 \left( 1 - |U_{\mu 3}|^2 \right) \sin^2 \Delta_{31}, \quad (25)$$

which yields

$$P(\nu_\mu \rightarrow \nu_\mu) \approx 1 - \sin^2 2\theta_{24} \sin^2 \Delta_{31}. \quad (26)$$

This implies that  $\sin^2 2\theta_{23}^{\text{eff}} = \sin^2 2\theta_{24}$ , so at 90% C.L., the region  $0.35 < \sin^2 \theta_{24} < 0.66$  cannot be excluded. This is the origin of the small non-excluded island at  $\Delta m_{41}^2 \approx 5 \times 10^{-3} \text{ eV}^2$  in Figure 21 (left).

$$\mathbf{C.} \quad \Delta m_{41}^2 = \Delta m_{31}^2$$

When  $\Delta m_{41}^2 = \Delta m_{31}^2$ ,  $\Delta m_{43}^2 = 0$ . On Figure 21, this corresponds to the region  $\Delta m_{41}^2 \approx 2.5 \times 10^{-3} \text{ eV}^2$ . This simplifies Equation 3 to:

$$P(\nu_\mu \rightarrow \nu_\mu) \approx 1 - 4 \left( |U_{\mu 3}|^2 + |U_{\mu 4}|^2 \right) \left( 1 - |U_{\mu 3}|^2 - |U_{\mu 4}|^2 \right) \sin^2 \Delta_{31} \quad (27)$$

Both the quasi-degeneracy and reactor degeneracy produce valid degenerate solutions. The quasi-degenerate case yields:

$$P(\nu_\mu \rightarrow \nu_\mu) \approx 1 - (1 - \sin^4 \theta_{24}) \sin^2 \Delta_{31}, \quad (28)$$

which implies that  $\sin^2 2\theta_{23}^{\text{eff}} = 1 - \sin^4 \theta_{24}$ , so at 90% C.L. the  $\sin^2 \theta_{24} > 0.33$  region is excluded. The reactor degenerate case yields:

$$P(\nu_\mu \rightarrow \nu_\mu) \approx 1 - \sin^2 2\theta_{24} \sin^2 \Delta_{31}, \quad (29)$$

so that at 90% C.L., the region  $0.35 < \sin^2 \theta_{24} < 0.66$  is not excluded. Since this limiting case only has terms proportional to  $\sin^2 \Delta_{31}$ , it is possible to extend the quasi-degenerate allowed region to smaller  $\sin^2 \theta_{24}$  values by allowing solutions with  $\sin^2 2\theta_{23} < 1$ . Considering all of these effects, at 90% C.L. the region  $\sin^2 \theta_{24} > 0.66$  is excluded.

#### D. $\Delta m_{41}^2 \rightarrow 0$

When  $\Delta m_{41}^2 \rightarrow 0$ ,  $\Delta m_{43}^2 \rightarrow -\Delta m_{31}^2$ . On Figure 21, this corresponds to the region  $\Delta m_{41}^2 < 1 \times 10^{-3} \text{ eV}^2$ . This simplifies Equation 3 to:

$$P(\nu_\mu \rightarrow \nu_\mu) \approx 1 - 4|U_{\mu 3}|^2 \left(1 - |U_{\mu 3}|^2\right) \sin^2 \Delta_{31}. \quad (30)$$

Both the quasi-degeneracy and atmospheric degeneracy produce valid degenerate solutions, and they are the same as the solutions in the  $\Delta m_{41}^2 = \Delta m_{31}^2$  case:  $\sin^2 2\theta_{23}^{\text{eff}} = 1 - \sin^4 \theta_{24}$  and  $\sin^2 \theta_{23}^{\text{eff}} = \sin^2 2\theta_{24}$ . Using the same reasoning as in the previous case, this produces a 90% C.L. excluded region for  $\sin^2 \theta_{24} > 0.66$ .

In all four limiting cases, the analysis of degenerate solutions provide 90% C.L. sensitivities in excellent agreement with the shape-only Asimov sensitivity using a full 3+1 flavor fit shown in Figure 21 (left).

## VII. LIMITATIONS OF ASIMOV SENSITIVITIES

A typical procedure for determining the sensitivity of an analysis is to construct a confidence interval using fake data derived from a high-statistics null-hypothesis prediction with nominal values of systematic parameters, scaled to the expected statistics of the data sample. This fake data is known as the Asimov sample and it represents the median experiment of a set of statistically and systematically fluctuated fake experiments. The resulting sensitivity is known as an Asimov sensitivity and is often assumed to be an approximation of the median sensitivity [2]. For this analysis, we have shown that Asimov sensitivities, for the shape + rate, shape-only, and rate-only fits, are in good agreement with our expectations in limiting cases where it is possible to predict the 90% C.L. sensitivity manually. However, the median sensitivity, computed from an ensemble of sensitivities derived from statistically and systematically fluctuated fake experiments, is generally a better estimate of the true sensitivity of an analysis.

To understand why this is, we first note that the Asimov sensitivity is produced with all systematic parameters set to zero. In any fit to data, it is highly unlikely that the fit would not choose shifted systematic parameters. Therefore, it is critical to explore how the sensitivity changes in the presence of fluctuations. In general, the Asimov sample will only approximate the median sensitivity well if symmetric fluctuations about the Asimov sample produce symmetric shifts about the Asimov sensitivity. This can be tested by applying positive and negative symmetric shifts to the Asimov sample with the shape of the full set of systematic uncertainties added in quadrature, as shown in Figure 23 (left). The sensitivities corresponding to the symmetrically shifted samples are shown in Figure 23 (right). The fluctuated sensitivities are not symmetric about the Asimov sensitivity, and the median point between the resulting sensitivity bands is consistently to the left of the Asimov sensitivity. Therefore, the Asimov sensitivity is not a reliable approximation of the median sensitivity. That is, the median spectrum does not necessarily yield the median sensitivity. Recently, this has been reported by other experiments as well. The joint LHC statistics committee has found that the median  $\chi^2$  value is consistently one unit larger than the  $\chi^2$  value for the Asimov sample when producing two-dimensional sensitivities. This means that the median sensitivity is always more stringent than the Asimov sensitivity [32]. The KM3NeT experiment has seen similar behavior in projecting future sensitivities for the neutrino mass ordering [33].

### A. Toy Monte Carlo Studies

We studied the behavior of fluctuated sensitivities using a toy Monte Carlo to better understand this effect. In these studies, the Asimov sample consisted of a histogram with 10 bins, each containing 100 events, and each bin was assigned a 20% systematic uncertainty. In the first version of this study, we generated covariance matrices with

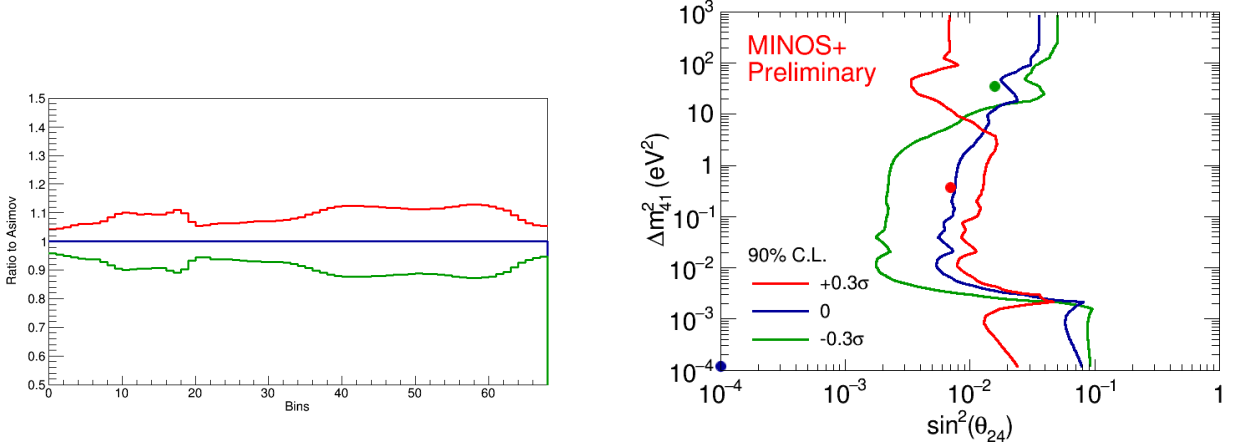

Figure 23. The ratio of systematically shifted fake data to the Asimov sample for a symmetrical shifts (left) and the resulting sensitivities for the Asimov sample and the positive and negative shifted samples (right). The solid circles are the best fit points. Shifts were performed for both the ND and FD according to the expected correlations between bins and detectors. Even though the systematic shifts are symmetrical about the Asimov sample, the resulting sensitivities are not symmetrical about the Asimov sensitivity.

random correlations between bins. We start with random correlations to determine whether or not the median shift we observe in the main analysis is due to the particular correlations encoded in the analysis covariance matrices. For each random covariance matrix, we fit a normalization-only physics model to the Asimov sample. This was performed in two modes: in disappearance mode, we only permitted normalization shifts which decreased the overall event count, and in appearance mode, we only permitted normalization shifts which increased the overall event count. We then randomly fluctuated the Asimov sample according to the systematic and statistical uncertainties encoded in the covariance matrix and performed disappearance and appearance normalization fits. For each randomly generated covariance matrix and fluctuated sample, we compute the asymmetry between the sensitivity computed using the fluctuated sample and the Asimov sensitivity. If the median of the asymmetry distribution is zero, there is no shift between the median and Asimov sensitivities.

Figure 24 (left) shows the asymmetry between the 90% C.L. sensitivities produced using the fluctuated samples and the Asimov sensitivities. This shows that fluctuated sensitivities tend to be more constraining than the Asimov sensitivity when fitting a disappearance model while the opposite is true for fits using an appearance model. The difference between appearance and disappearance is due to the fact that although the relative error covariance matrices used in the fits remain the same, they have to be scaled to the predicted spectrum to produce absolute error covariance matrices. MiniBooNE previously scaled their relative error covariance matrices iteratively between fits [34]. Since we perform it dynamically inside the MINUIT [35] objective function, we call this process *dynamic scaling*. Disappearance fits tend to produce smaller absolute errors than appearance fits. Figure 24 (right) shows the same asymmetry distributions computed with dynamic scaling turned off. In this case the median asymmetry, and thus, the difference between the median and Asimov sensitivities, in both modes becomes very small. However, it is critical to note that failing to dynamically scale the covariance matrices in the fit is statistically incorrect.

Next, we examined whether any particular correlation structure maximized the asymmetry between fluctuated and Asimov sensitivities. As seen in Figure 25 (left), we found that covariance matrices with 100% correlations between bins produced much larger asymmetries than those produced by matrices with random correlations. This is an example where the physics model (a normalization) is degenerate with the systematic uncertainty (a matrix with flat, fully-correlated uncertainties). In Figure 25 (right), we continue to use 100% correlated covariance matrices, but the fluctuated samples are constructed only using statistical fluctuations. The observed asymmetries remain as large as in the case where the samples were fully fluctuated.

We then checked cases where the systematic uncertainties are not degenerate with the physics model. In Figure 26 (left), the systematic uncertainties are fully uncorrelated and act like excess statistical uncertainties in each bin, but the physics model being fit is a normalization shift. This produces median asymmetries that are smaller than the fully correlated case. In Figure 26 (right) we fit a linear physics model, where the shift linearly increases with bin number, using matrices with flat, fully-correlated uncertainties, and we find a large reduction in the median asymmetry.

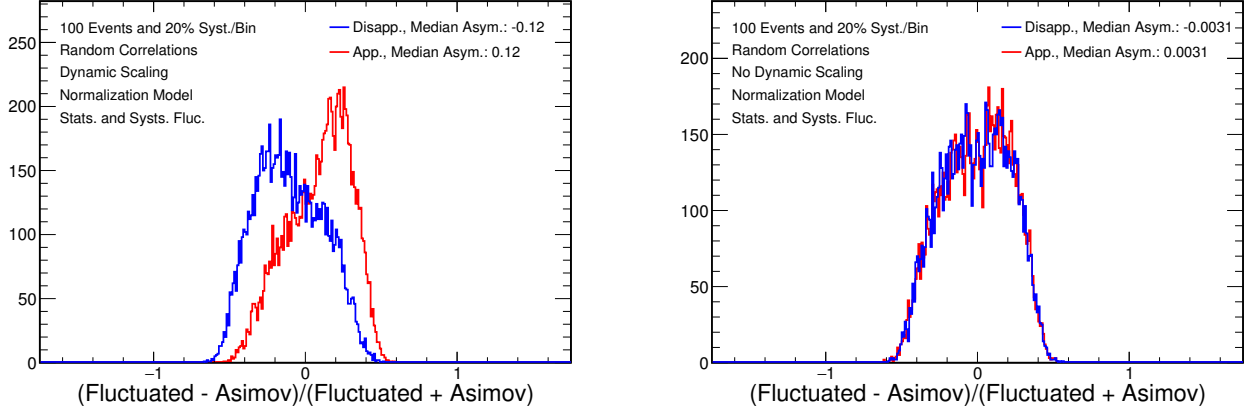

Figure 24. The distribution of the asymmetry between fluctuated sensitivities and Asimov sensitivities for appearance (red) and disappearance (blue) mode. (Left) Using covariance matrices with a constant 20% systematic uncertainty per bin, but with random bin-to-bin correlations. The fluctuated and Asimov samples were fit using a normalization model in either appearance or disappearance mode. In disappearance mode, fluctuated sensitivities tend to be more constraining than Asimov sensitivities. (Right) Using covariance matrices with a constant 20% systematic uncertainty per bin, but with random bin-to-bin correlations and dynamic scaling turned off. In this case, the median asymmetry is very small in both disappearance and appearance modes.

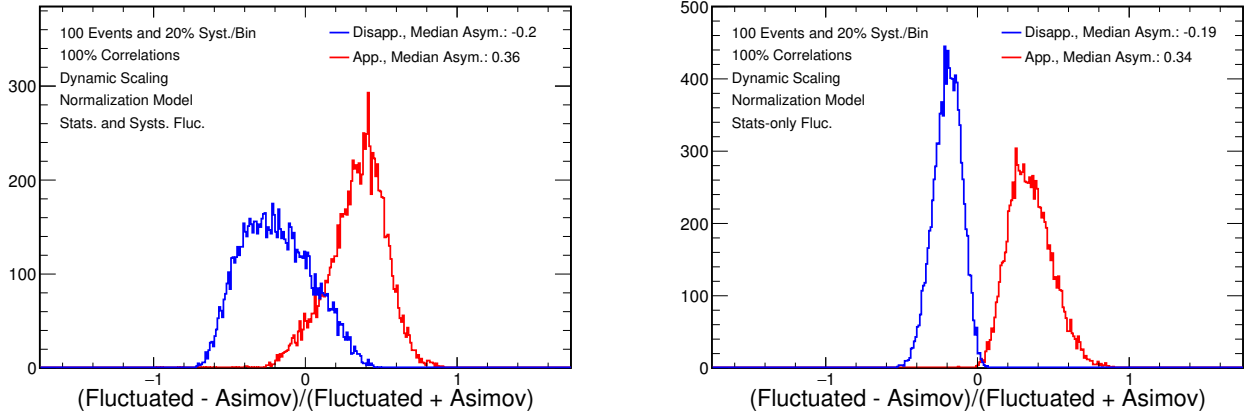

Figure 25. The distribution of the asymmetry between fluctuated and Asimov sensitivities in appearance (red) and disappearance (blue) mode using a toy model where samples are fit to a normalization model using fully correlated systematic uncertainties. (Left) The fluctuated samples are varied according to both statistical and systematic uncertainties. (Right) The fluctuated samples are varied only according to statistical uncertainties.

## B. Fluctuating Systematic Categories

Based on the results from the toy model, we next test the hypothesis that large shifts in the median sensitivity relative to the Asimov sensitivity occur when there is a degeneracy between the physics being fit and the shape of the systematic uncertainties, and uncorrelated uncertainties are present. We perform this test by constructing median sensitivities using the full analysis framework and covariance matrices, but we only include a subset of uncertainties in the fluctuations.

In Figure 27 (left), we see the median constructed by fluctuating only statistical uncertainties. In the FD dominated region, this explains the entire median shift, but in the ND dominated region, it only explains about half of the median shift. This makes sense since the fractional statistical uncertainty is very small in the ND, where event rates are high. To explain the remainder of the median shift in the ND dominated region, we fluctuate both statistical uncertainties and the acceptance systematic uncertainties, as seen in Figure 27 (right). The acceptance uncertainties, as shown in Section III, are uncorrelated, only calculated for the ND, and large compared to the statistical uncertainty.

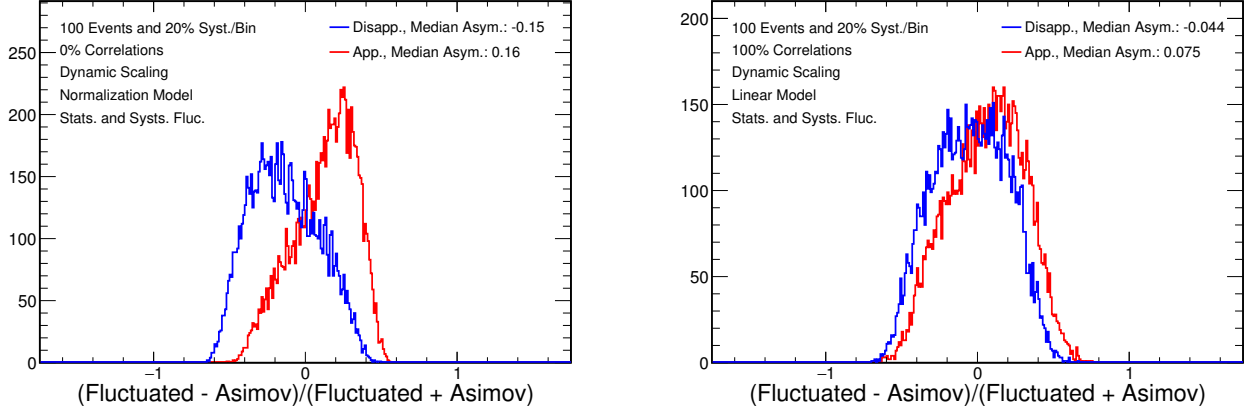

Figure 26. The distribution of the asymmetry between fluctuated and Asimov sensitivities in appearance (red) and disappearance (blue) mode using a toy model. (Left) Fit to a normalization using fully uncorrelated systematic uncertainties. (Right) Fit to a linear model, where the size of the shift grows linearly by bin, using fully correlated systematic uncertainties.

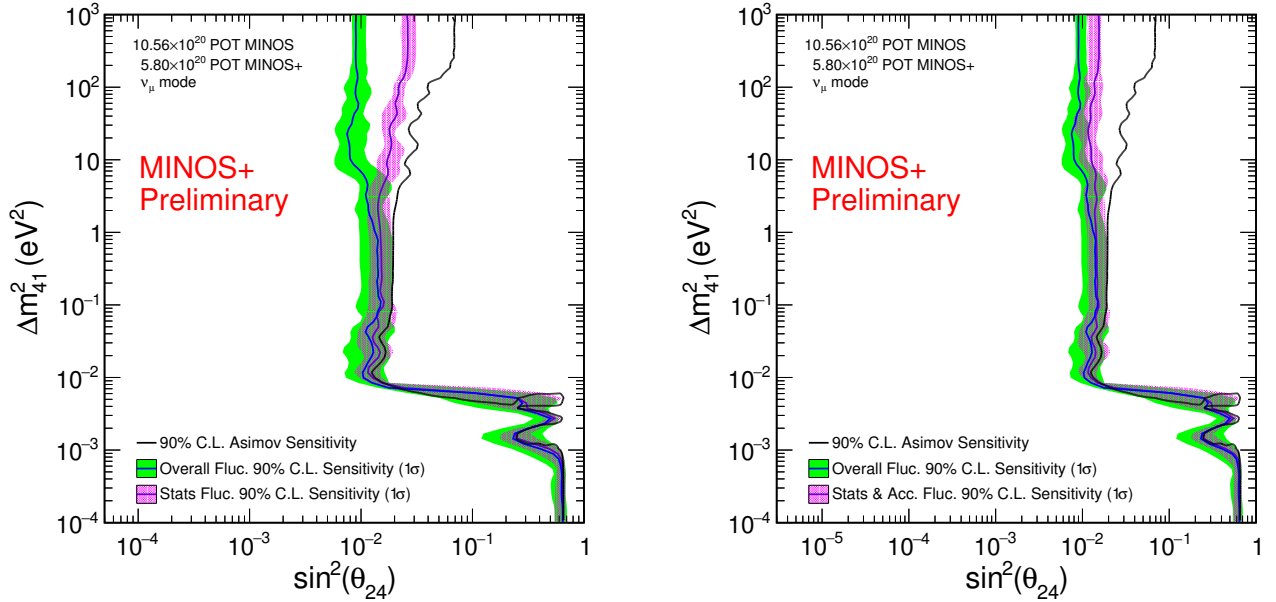

Figure 27. A comparison of the Asimov sensitivity and the median sensitivity after varying statistics (left) and statistics + acceptance systematic uncertainties (right).

### C. Asimov and Median Scaling

Since the median shift is driven both by systematic uncertainties that are degenerate with the physics model and uncorrelated uncertainties, it is natural to be concerned that median sensitivity inappropriately rewards large systematic uncertainties or low statistics. To confirm that this is not true, a study was performed where the Asimov sensitivity was compared to an ensemble of 400 fluctuated sensitivities with nominal statistics and the full analysis covariance matrix. This study was then repeated with a factor of 400 higher statistics and a with a factor of 4000 lower statistics, as well as with the analysis systematic uncertainty covariance matrix scaled between 0% (which represents a statistics-only fit) and 200%. Figure 28 shows how the Asimov (left) and median (right) sensitivities at  $\Delta m^2_{41} = 500 \text{ eV}^2$  change in each case. As the scale of the systematic uncertainties increases, both the Asimov and median sensitivities become weaker, as expected. For the statistics-only case, both sensitivities become stronger as the statistics increase. As the systematic scale increases, the nominal and increased statistics samples converge to

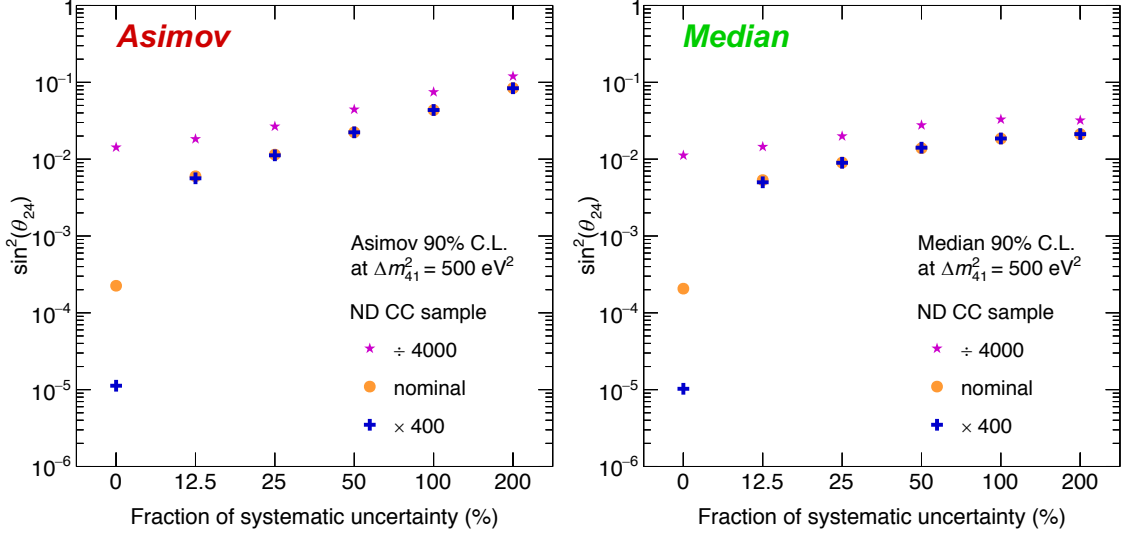

Figure 28. Behavior of the Asimov sensitivity (left) and median sensitivity (right) as a function of a scaling of the analysis systematic uncertainty covariance matrix – ranging from 0% (i.e. statistical uncertainties only) to 200% – for nominal statistics (orange), statistics decreased by a factor of 4000 (magenta), and statistics increased by a factor of 400 (blue) ND CC sample.

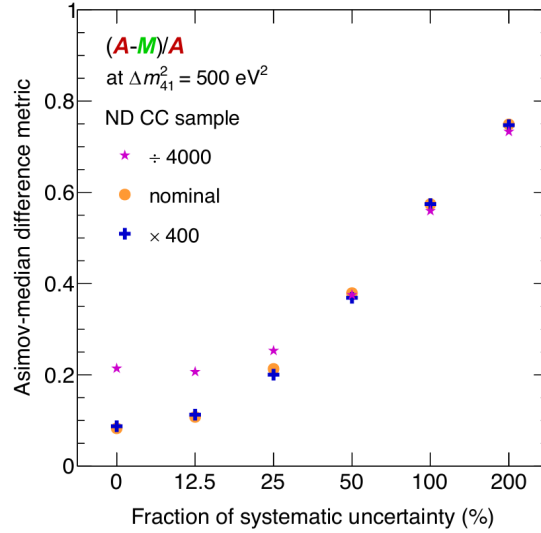

Figure 29. Quantifying the difference between the Asimov and median using  $(A - M)/A$ . We define  $A$  to be the Asimov sensitivity and  $M$  to be the median sensitivity at  $500 \text{ eV}^2$ . The  $(A - M)/A$  metric is a measure of the fractional difference between the Asimov and median sensitivities.

the same sensitivities indicating that those cases are systematically limited. The reduced statistics sample remains weaker than the other two at all systematic uncertainty scales.

Figure 29, compares the Asimov and median sensitivities using the  $(A - M)/M$  metric, the measure of the fractional difference between the Asimov and median sensitivities. As the systematic uncertainty scale increases, the Asimov sensitivity weakens faster than the median sensitivity, which corresponds to an increase in the fractional difference. In the limit of high statistics and low systematic uncertainties, the fractional difference comes close to zero. This is consistent with our previous observations that systematic uncertainties which are degenerate with the effect of the physics being fit exacerbates the difference between the Asimov and median sensitivities, but that uncorrelated uncertainties, like statistical uncertainties, are necessary to produce the deviation.

In summary, these three studies, taken together, indicate that under even very simple circumstances, the median sensitivity does not agree with the Asimov sensitivity. Due to dynamic scaling effects on the absolute uncertainty, the

median sensitivity is generally stronger than the Asimov sensitivity in the case of disappearance, but the situation is reversed in the case of appearance. The maximum effect occurs when the systematic uncertainties are degenerate with the physics model being fit, and an uncorrelated component is present. The median sensitivity behaves intuitively in that it becomes weaker in the presence of increased systematic uncertainties, and it becomes stronger as the sample size increases; however, the median sensitivity degrades with increased systematic uncertainties slower than the Asimov sensitivity does. All indications suggest that the median is a more complete measure of sensitivity than the Asimov since it accounts for the range of shape changes allowed due to systematic variation, and it correctly accounts for changes due to dynamic scaling.

### VIII. FITTER ASSUMPTIONS

In our nominal fit,  $\theta_{23}$ ,  $\theta_{24}$ ,  $\theta_{34}$ ,  $\Delta m_{31}^2$ , and  $\Delta m_{41}^2$  are allowed to freely vary. The solar parameters are set at values of  $\sin^2 \theta_{12} = 0.307$  and  $\Delta m_{21}^2 = 7.54 \times 10^{-5} \text{ eV}^2$ , based on a three-flavor global fit [36], and we fix  $\sin^2 \theta_{13} = 0.02213$  [37]. The other parameters of the 3+1 model,  $\theta_{14}$  and the CP-violating phases,  $\delta_{13}$ ,  $\delta_{14}$ , and  $\delta_{24}$  are fixed to zero.

To verify that our sensitivity to  $\theta_{14}$  is minimal, we performed an alternate fit with  $\theta_{13}$  and  $\theta_{14}$  free, but taking into account strong constraints on these parameters. In the case where  $\Delta m_{41}^2$  is sufficiently larger than  $\Delta m_{31}^2$ ,  $|U_{e4}|$  is constrained by unitarity considerations, which imply  $\sin^2 \theta_{14} < 0.036$  at  $1\sigma$  [38]. In the degenerate case,  $\theta_{14}$  is constrained by measurements of  $\theta_{13}$  [37], and  $\theta_{13} = \pi/2$ . As shown in Figure 30, the changes in the resulting Asimov sensitivity and non-Feldman-Cousins corrected data limit are negligible. A similar study where all CP-violating phases were allowed to freely vary showed negligible changes to the limit and sensitivity.

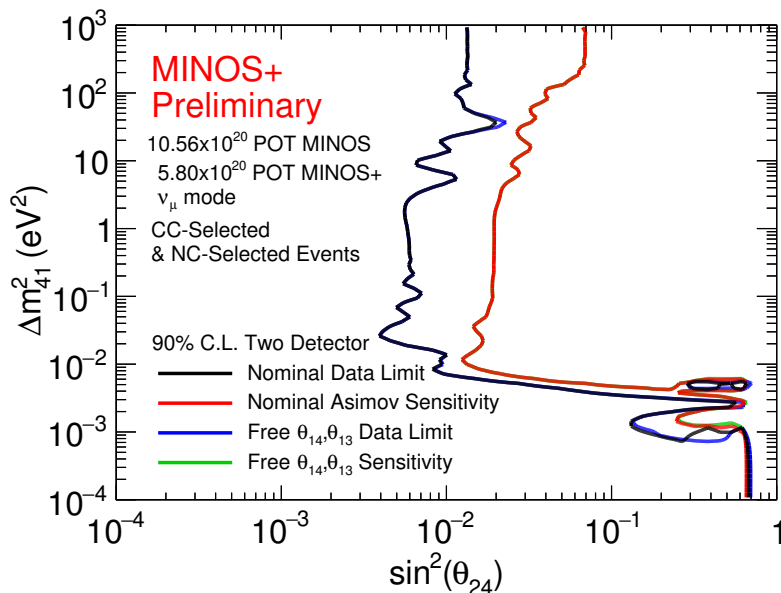

Figure 30. A comparison of how the Asimov sensitivity and non-Feldman-Cousins corrected data limit change if  $\theta_{14}$  is allowed to vary. Unitarity constraints require  $\theta_{14}$  to be small. The blue curve is underneath the black curve, and the green is underneath the red.

Finally, for computational purposes, we neglect matter effects in computing oscillation probabilities. To determine the effect this has on the data limit, we computed the  $\chi^2$  profile as a function of  $\sin^2 \theta_{24}$  at a series of fixed  $\Delta m_{41}^2$  values. As shown in Figure 31, neglecting the matter effect either does not change the data limit, or it is conservative.

### IX. RESULTS AND DISCUSSION

The reconstructed energy spectra of data collected by the combined MINOS and MINOS+ experiments for CC selected and NC selected events after application of the decorrelation procedure are shown in Figures 32 and 33, respectively. A comparison of the data spectra with the three-flavor prediction spectra shows no significant modulations

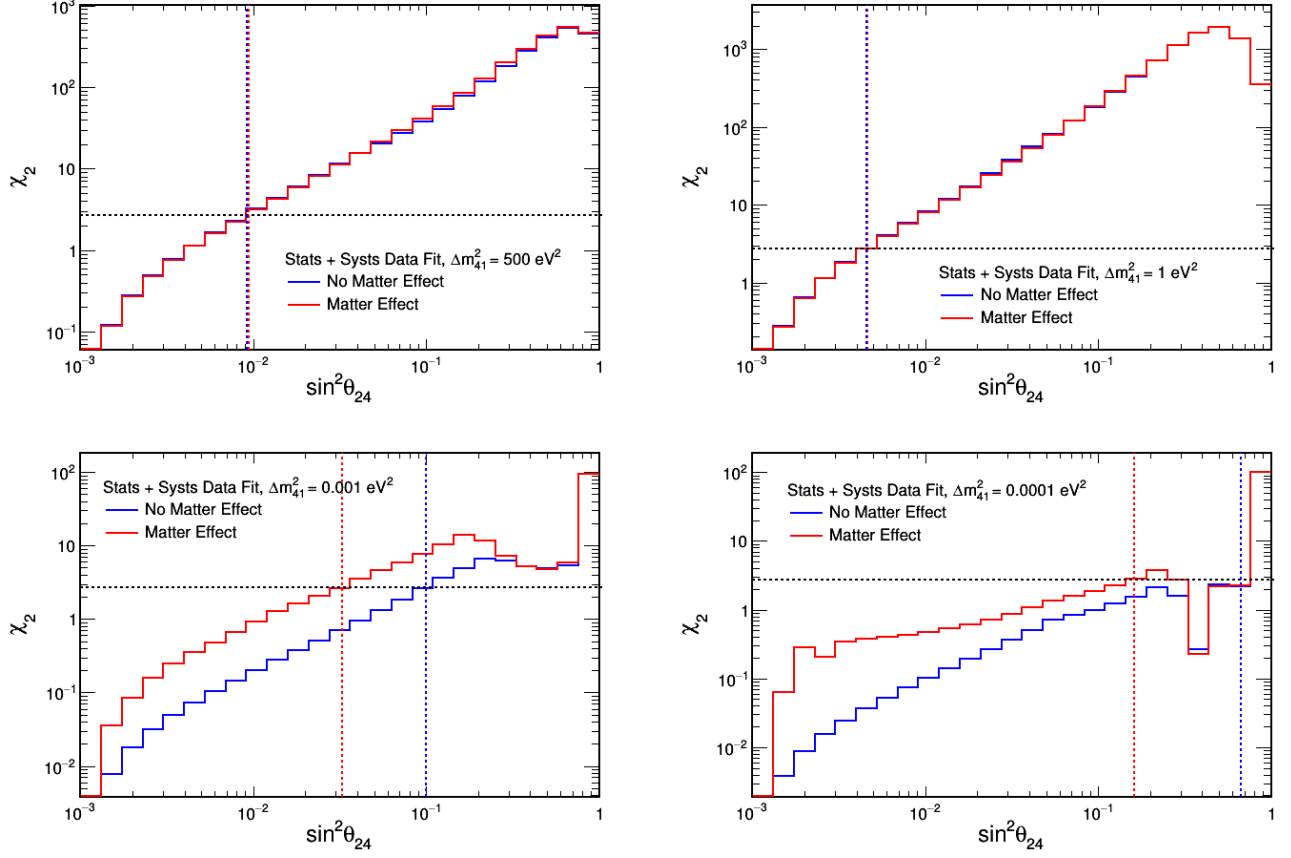

Figure 31. A study of how the data limit changes for  $\Delta m_{41}^2$  at 500 eV<sup>2</sup> (top left), 1 eV<sup>2</sup> (top right), 0.001 eV<sup>2</sup> (bottom left), and 0.0001 eV<sup>2</sup> (bottom right) if the matter effect is taken into account. In all cases, neglecting the matter effect either does not change the limit, or it is conservative.

consistent with a 3+1-flavor model. Fluctuations are observed between data and MC simulation which are consistent with those expected from statistical and systematic uncertainties. The best fit values for the sterile mixing values were determined to be  $\Delta m_{41}^2 = 0.0023$  eV<sup>2</sup> and  $\sin^2(\theta_{24}) = 0.0001$ , with a best fit  $\chi_{\min}^2 = 99.308$  (140 degrees of freedom), which represents a negligible deviation from the case of three-flavor oscillations ( $\chi_{\min}^2 = 99.3085$ , as illustrated by the coincidence of the three-flavor and 3+1-flavor predictions). Having detected no significant evidence for neutrino oscillations mediated by the existence of a sterile neutrino state in a 3+1-flavor model, we set a confidence interval at the 90% C.L. in the  $\Delta m_{41}^2$ - $\sin^2(\theta_{24})$  parameter space, which is plotted in the Figure 34.

#### A. Comparison of the Data Limit with Expected Sensitivity

The exclusion contour derived from the data fit has two distinct regions of differing behavior, predominantly corresponding to the ND and FD, as shown in Figure 18, which merit further explanation. To understand the empirical likelihood of observing our limit, we simulate pseudo-experiments that are systematically and statistically varied according to the constraints encoded in the covariance matrix, and we construct a 90% CL sensitivity for each fluctuated experiment. As outlined above, the median sensitivity of the fluctuated pseudo-experiments is more constraining than the Asimov sensitivity as expected in the case of our systematically dominated, highly correlated covariance matrix fit, and this is in fact the appropriate sensitivity to expect from conducting our search. In the FD dominated region, where  $\Delta m_{41}^2 \leq 3$  eV<sup>2</sup>, the data contour is more constraining at 90% C.L. than the predicted sensitivity, which may be attributed to the excess event rate observed in the FD spectrum seen in Figure 32. Such FD fluctuations are consistent with our estimated statistical and systematic uncertainties found in the covariance matrix as evidenced by the observation that the data exclusion contour has limited excursions beyond the  $1\sigma$  fluctuated sensitivity band.

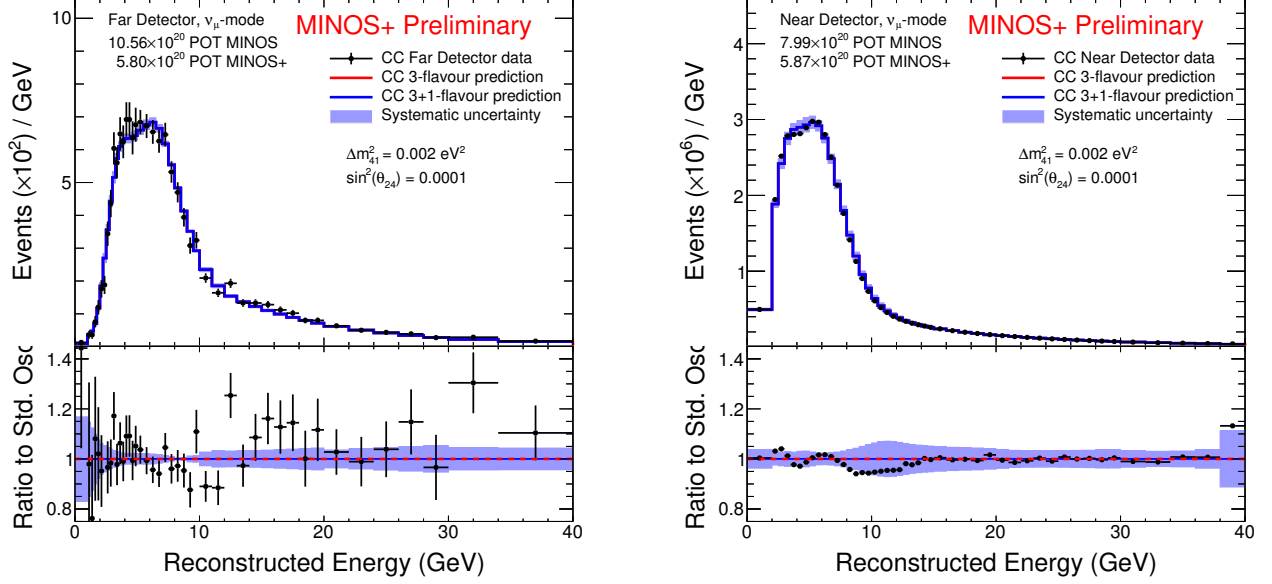

Figure 32. The FD CC selected sample (left) and the ND CC selected sample (right) compared to MC with three-flavor oscillations (red) and the best fit 3+1-flavor prediction (blue) after correcting the prediction using the covariance matrix decorrelation procedure.

The juxtaposition of the ND and FD dominated regions shows clear opposite behavior for the ND wherein the data limit excludes less parameter space than would have generally been anticipated. The conservative limit in the ND region is caused by the application of the beam fit procedure and resulting flux correction as described in previous sections. The modifications to the flux made by the effective PPFX parameterization in the 0-20 GeV range are small effects in comparison with a large shift in the normalization of expected events in the tail region. Given that this flux correction does not correspond with any of the shape behaviors of the known systematic uncertainties, the limit shows an apparent rightward fluctuation with a  $\sim 1\sigma$  excursion from the expected sensitivity. Rather than evidence for a sterile neutrino oscillations signal, this points to the extreme conservatism of the limit derived from our beam fit flux correction method.

### B. Significance of the FD Neutral Current Excess

As seen in Figure 3, the peak of the NC sample in the FD agrees well with the prediction while there is a small deficit of NC events in the peak in the ND compared with the prediction. A concern was raised that this might be a hint for appearance between the ND and FD, and thus, for new physics. Since almost all  $\nu_e$  at the FD are selected as NC events, the concern was that this could be due anomalous  $\nu_e$  appearance. To assess this, we determined the data/MC ratio for the FD and ND and constructed the double ratio of the FD ratio and the ND ratio, as seen in Figure 35.

Double ratios from the CC and NC samples are compared to systematic uncertainty bands which properly account for correlations between the ND and FD encoded in the covariance matrix. In the CC sample, systematic variations seen in Figure 2 fully cancel, and the p-value, the probability of observing a double ratio spectrum under the no sterile hypothesis with greater disagreement than our data, is 0.418. In the NC sample, the double ratio is systematically high. However, due to the large statistical and systematic uncertainties for the NC sample, the p-value is 0.999, indicating that the NC sample is actually in greater agreement with the no sterile hypothesis than the CC sample.

### C. Oscillations at Large Mass Splittings

At high  $\Delta m^2_{41}$ , the 90% C.L. limit on  $\sin^2 \theta_{24}$  is  $\sim 0.025$ . Using the short-baseline approximation and a counting experiment  $\chi^2$ , described in Section V, one could conclude our normalization uncertainty is  $\sim 3\%$ ; however, we have

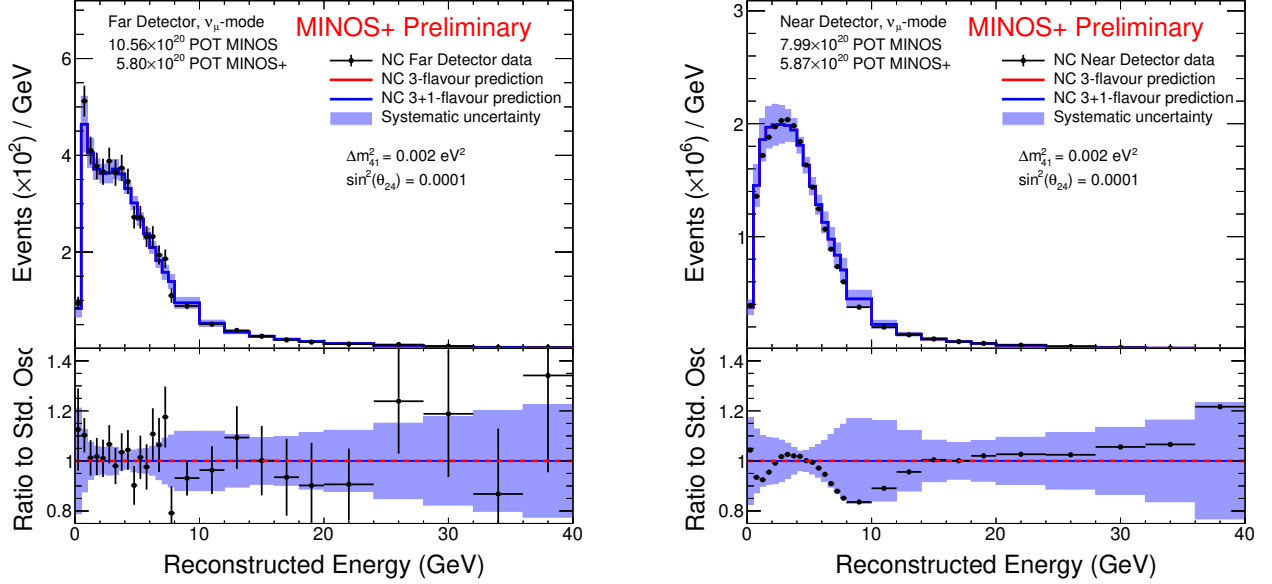

Figure 33. The FD NC selected sample (left) and the ND NC selected sample (right) compared to MC with three-flavor oscillations (red) and the best fit 3+1-flavor prediction (blue) after correcting the prediction using the covariance matrix decorrelation procedure.

shown that the normalization uncertainty of the CC sample is between 8.3% and 10.3%, depending on the method used to extract the normalization component from the full uncertainty. Regardless, we have demonstrated that shape + rate, shape-only, and normalization-only Asimov sensitivities all perform as expected, which indicates that there is nothing wrong with the systematic uncertainties used in the analysis covariance matrices or the fit methodology as a whole. Instead, we found that sensitivities performed on statistically and systematically fluctuated samples tend to exclude more parameter space than the Asimov sensitivities. We have found that this occurs in very generic circumstances, including in very simplified toy models. These observations imply that the shape of the signal being fit is not the only source of shape in this analysis. Indeed, shape information induced by fluctuations are critical and not captured by the Asimov procedure. A median sensitivity accounts for these shapes by examining an ensemble of sensitivities produced with fluctuations that could plausibly occur in the data and constructing a representative contour that summarizes the behavior of the ensemble. As shown in Figure 34, the data limit is in good agreement with the median sensitivity.

To make explicit the calculations underpinning our data contour for high  $\Delta m_{41}^2$ , we present the full result underlying the  $\chi^2$  surface at a test point where  $\Delta m_{41}^2 \approx 1000 \text{ eV}^2$  and  $\sin^2(\theta_{24}) = 0.039$ . The CC reconstructed energy spectra at the test point are shown in Figure 36 and the NC reconstructed energy spectra are plotted in Figure 37 both for correlated and decorrelated systematic uncertainties. The  $\chi^2$  and  $\Delta\chi^2$  contributions arising from these reconstructed energy spectra are plotted in Figure 38 and Figure 39. From this test point in parameter space, it is shown that in an analysis with a large number of bins of reconstructed energy, as in the case of this sterile search, small  $\chi^2$  contributions from each bin can have a significant cumulative effect, though this of course does not preclude a few bins from having larger contributions than others. We can also see from the cumulative totals of the  $\chi^2$  contributions at this point that this set of parameters is robustly disfavored by the observed data.

## X. CONCLUSIONS

Due to the novelty of the methods used in the 2017 MINOS and MINOS+ sterile analysis [1] and the resulting world-leading data limits produced, we have performed in depth checks on every aspect of the analysis. Searching sterile neutrino driven oscillations at both short and long baselines simultaneously leverages the interplay of pure sterile oscillations at the ND and the interference between sterile and three-flavor oscillations at the FD. This interplay is subtle and critically depends on understanding shape effects. In fact, normalization effects are only important at very large  $\Delta m_{41}^2$  values, which are of less importance in the context of  $\nu_e$  anomalies seen at LSND and MiniBooNE. After

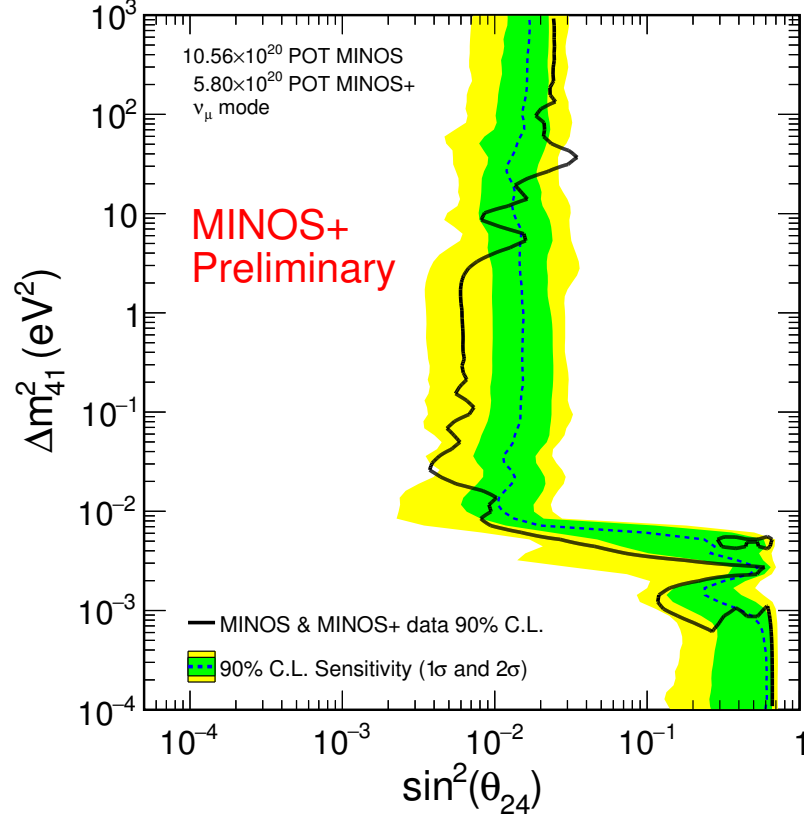

Figure 34. A comparison of sensitivity generated with statistically and systematically fluctuated predictions with the limit derived from data. At high  $\Delta m_{41}^2$ , most fluctuated predictions produce more stringent constraints than the observed data.

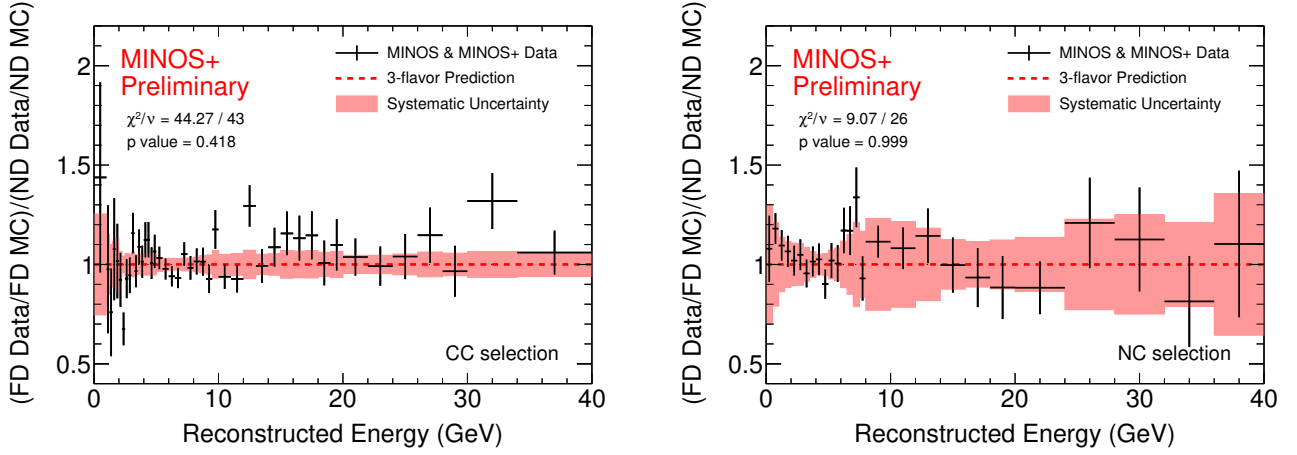

Figure 35. Left: CC double ratio. Right: NC double ratio.

detailed study, we have determined that this analysis is conservative and robust.

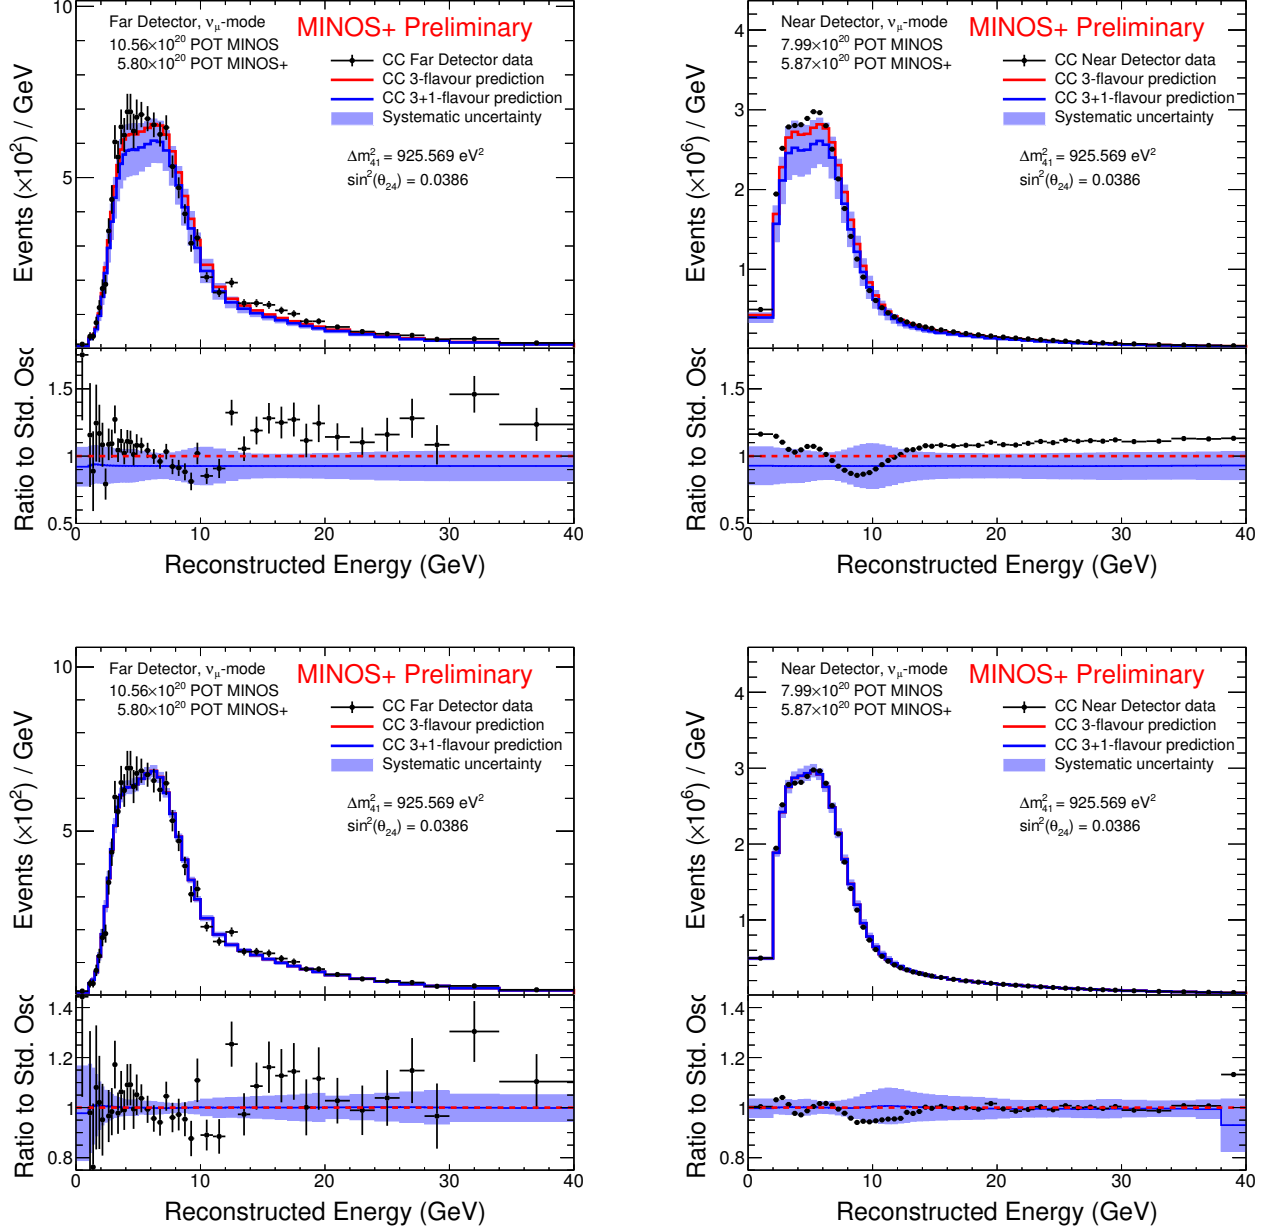

Figure 36. The MINOS and MINOS+ combined data FD CC selected sample (left) and the ND CC selected sample (right) compared to MC for an excluded test point in the parameter space where  $\Delta m_{41}^2 \approx 10^3 \text{ eV}^2$ . The top row shows the raw comparison while the bottom row shows the spectra after correcting the prediction using the covariance matrix decorrelation procedure.

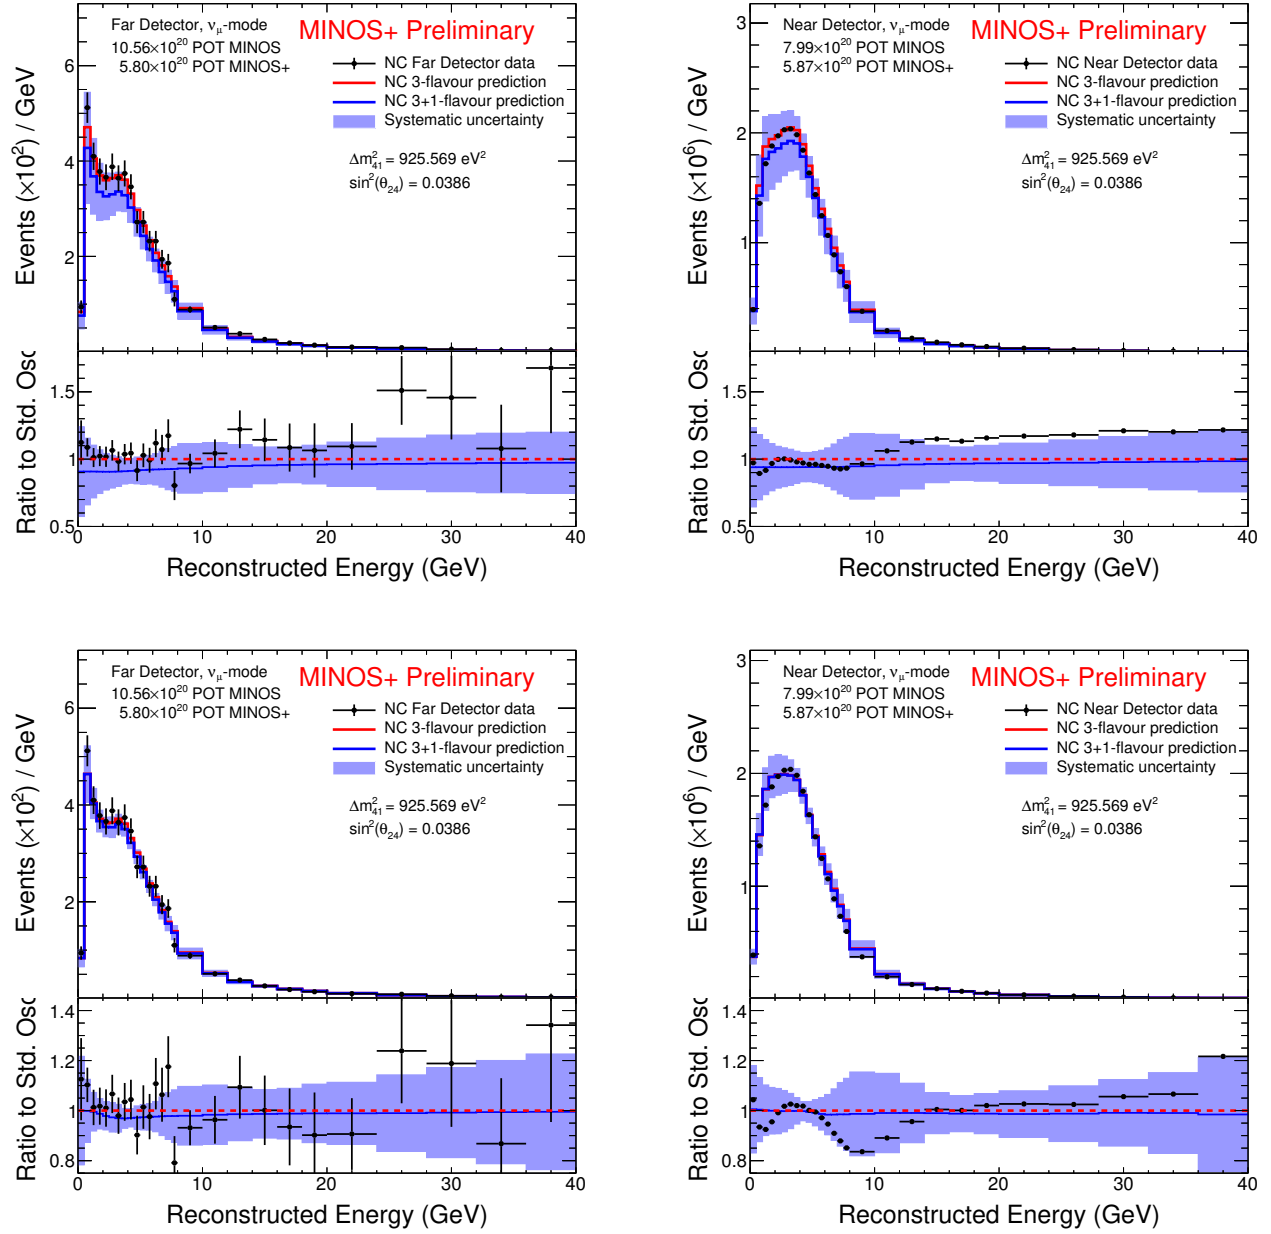

Figure 37. The MINOS and MINOS+ combined data FD NC selected sample (left) and the ND NC selected sample (right) compared to MC for an excluded test point in the parameter space where  $\Delta m_{41}^2 \approx 10^3 \text{ eV}^2$ . The top row shows the raw comparison while the bottom row shows the spectra after correcting the prediction using the covariance matrix decorrelation procedure.

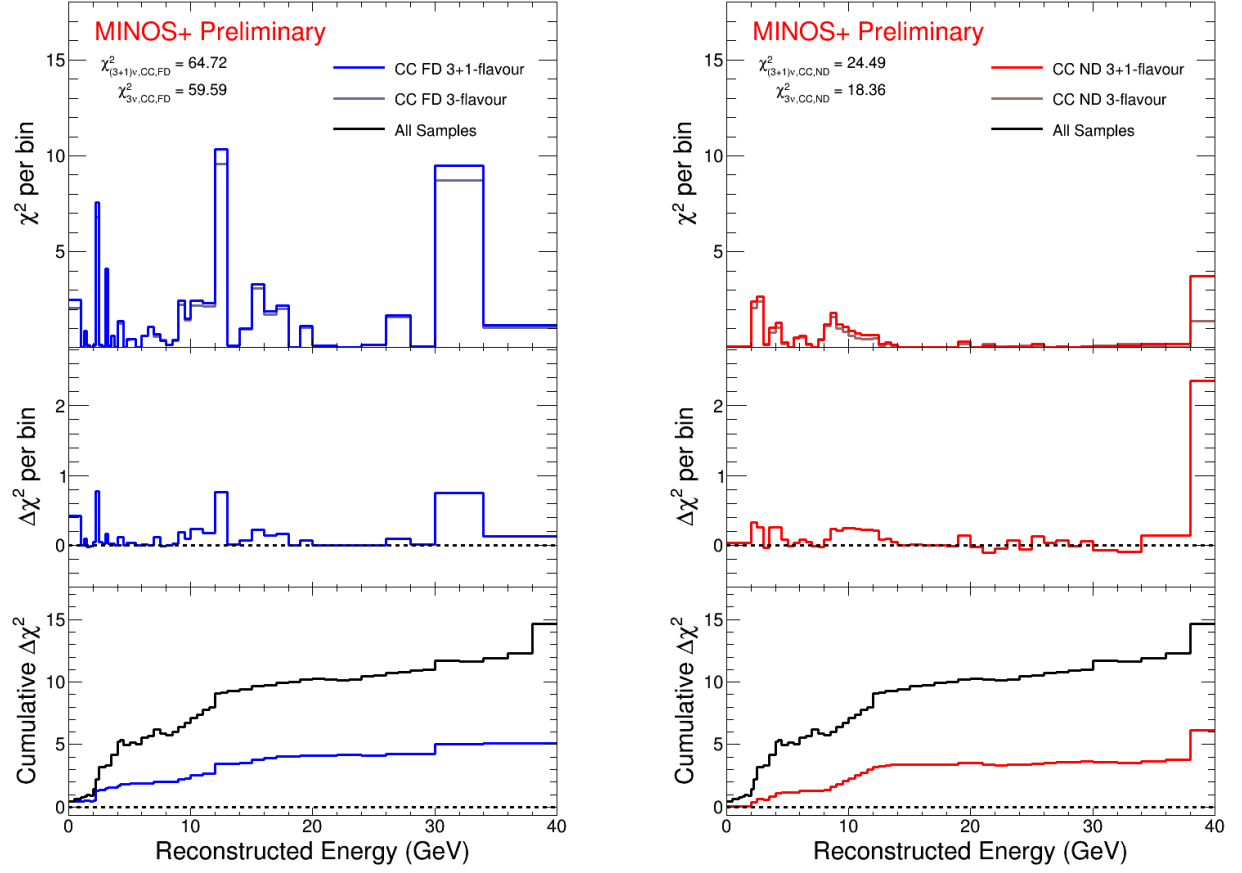

Figure 38. A summary of the contributions from the CC samples to the  $\chi^2$  statistic at the test point ( $\Delta m_{41}^2 = 925.69 \text{ eV}^2$ ,  $\sin^2 \theta_{24} = 0.0386$ ) from each of the energy bins of the MINOS and MINOS+ combined data spectrum at the point in parameter space used for Figure 36.

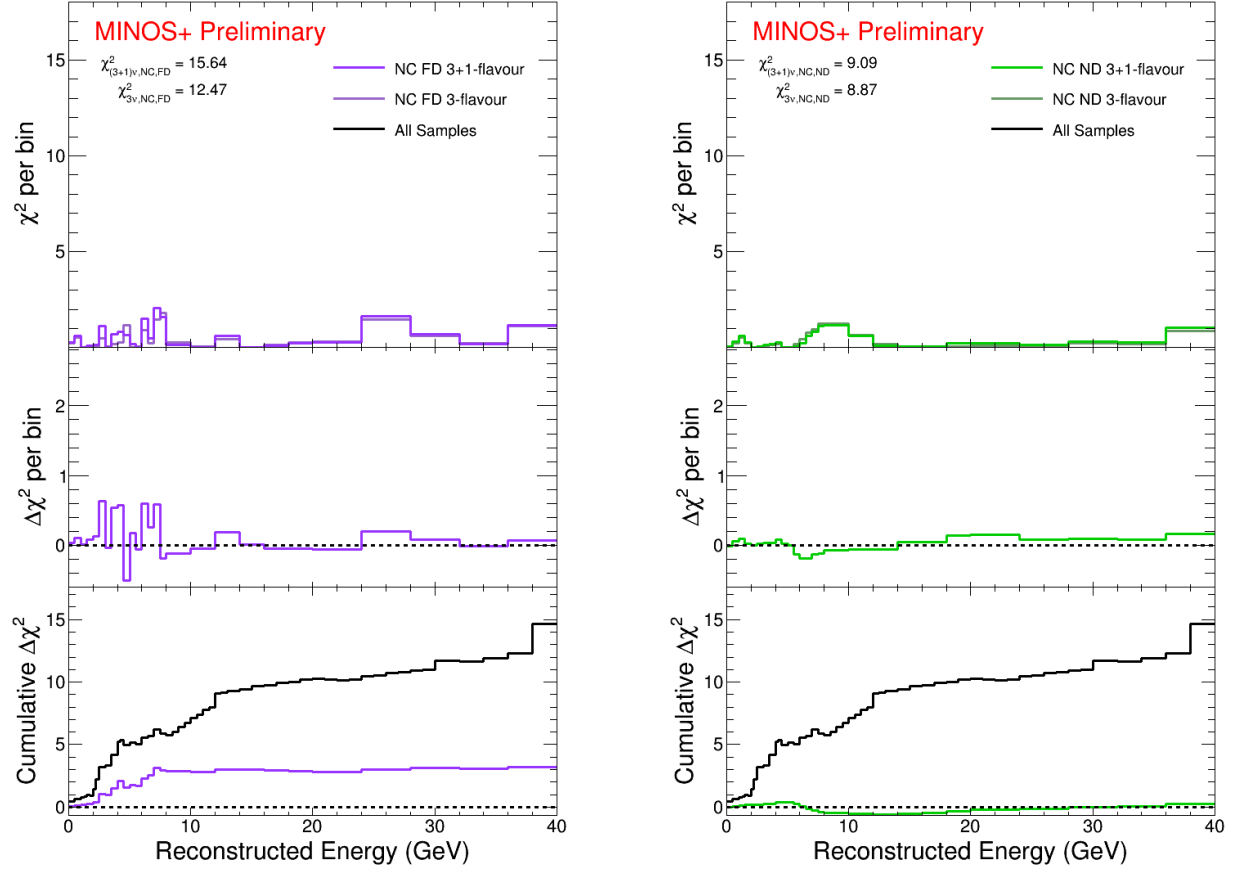

Figure 39. A summary of the contributions from the NC samples to the  $\chi^2$  statistic at the test point ( $\Delta m_{41}^2 = 925.69 \text{ eV}^2$ ,  $\sin^2 \theta_{24} = 0.0386$ ) from each of the energy bins of the MINOS and MINOS+ combined data spectrum at the point in parameter space used for Figure 37.

## Appendix A: Conditional Multivariate Gaussian Distributions

Performing a fit with a covariance matrix-based  $\chi^2$  function implies that the energy bins are distributed according to a multivariate Gaussian distribution. A multivariate Gaussian distribution is a generalization of the univariate Gaussian distribution, which consists of a set of normally distributed random variables that may or may not be correlated. In the event that the multivariate Gaussian is correlated, and thus covariances exist between the variables, one can compute the conditional distribution of a subset of the variables given the observation of the remaining subset.

Correlated systematic uncertainties are powerful, but they have a number of drawbacks. First, we normally use the square root of the diagonal terms of the covariance matrix to visualize the systematic uncertainty band. However, this can be misleading. Depending on the size of the off-diagonal terms, points well outside of the visualized uncertainty band may not induce a large  $\chi^2$  value. Second, although covariance matrices encode systematic uncertainties, they are not visibly corrected for in the fit in the way that a penalty term treatment would.

It is possible to solve both of these problems by calculating how the prediction for one set of bins would change if you observed a different subset. This is similar to the traditional extrapolation method which uses the data/MC disagreement at the ND to correct the FD prediction. This can be achieved in a covariance matrix fit by modeling a subset of the data as taken from a multivariate Gaussian distribution conditional on a different subset.

Consider multivariate Gaussian distribution,  $\mathbf{x} \sim N(\boldsymbol{\mu}, \boldsymbol{\Sigma})$  where  $\mathbf{x}$  contains  $N$  random variables representing histogram bins,  $\boldsymbol{\mu}$  is the nominal prediction, and  $\boldsymbol{\Sigma}$  is the positive semi-definite symmetric matrix describing the covariances between bins. The  $N$  bins can be partitioned into two group  $\mathbf{x}_1$  and  $\mathbf{x}_2$ , which could represent the FD bins and ND bins, such that

$$\mathbf{x} = \begin{bmatrix} \mathbf{x}_1 \\ \mathbf{x}_2 \end{bmatrix} \text{ with sizes } \begin{bmatrix} q \times 1 \\ (N - q) \times 1 \end{bmatrix} \quad (\text{A1})$$

with the mean vector given by

$$\boldsymbol{\mu} = \begin{bmatrix} \boldsymbol{\mu}_1 \\ \boldsymbol{\mu}_2 \end{bmatrix} \text{ with sizes } \begin{bmatrix} q \times 1 \\ (N - q) \times 1 \end{bmatrix} \quad (\text{A2})$$

and the covariance matrix taking the form

$$\boldsymbol{\Sigma} = \begin{bmatrix} \boldsymbol{\Sigma}_{11} & \boldsymbol{\Sigma}_{12} \\ \boldsymbol{\Sigma}_{21} & \boldsymbol{\Sigma}_{22} \end{bmatrix} \text{ with sizes } \begin{bmatrix} q \times q & q \times (N - q) \\ (N - q) \times q & (N - q) \times (N - q) \end{bmatrix} \quad (\text{A3})$$

Using the FD and ND example,  $\boldsymbol{\mu}_1$  is the nominal FD prediction and  $\boldsymbol{\mu}_2$  is the nominal ND prediction. Similarly  $\boldsymbol{\Sigma}_{11}$  is the FD covariance matrix,  $\boldsymbol{\Sigma}_{22}$  is the ND covariance matrix, and  $\boldsymbol{\Sigma}_{12}$  and  $\boldsymbol{\Sigma}_{21}$  contain covariances between the detectors.

Now consider an observation (measurement) is made of  $\mathbf{x}_2$  such that  $\mathbf{x}_2 = \boldsymbol{\alpha}$ . One can calculate the conditional distribution of  $\mathbf{x}_1$  after accounting for the correlations encoded in the covariance matrix. Calculating the FD distribution conditional on the ND is effectively an extrapolation procedure.

The conditional distribution is defined by  $\mathbf{x}_1 \sim N(\bar{\boldsymbol{\mu}}, \bar{\boldsymbol{\Sigma}})$  [39] where

$$\bar{\boldsymbol{\mu}} = \boldsymbol{\mu}_1 + \boldsymbol{\Sigma}_{12} \boldsymbol{\Sigma}_{22}^{-1} (\boldsymbol{\alpha} - \boldsymbol{\mu}_2) \quad (\text{A4})$$

with variance

$$\bar{\boldsymbol{\Sigma}} = \boldsymbol{\Sigma}_{11} - \boldsymbol{\Sigma}_{12} \boldsymbol{\Sigma}_{22}^{-1} \boldsymbol{\Sigma}_{21} \quad (\text{A5})$$

In a simple two bin example, after computing the conditional distribution of  $\mathbf{x}_1$ ,  $\mathbf{x}_1$  and  $\mathbf{x}_2$  are no longer correlated. In addition,  $\boldsymbol{\mu}_2$  is corrected according to the difference between  $\boldsymbol{\alpha}$  and  $\boldsymbol{\mu}_2$ . For more than two bin fits, this decorrelation procedure can be performed recursively, correcting  $N - 1$  based on observed data. This procedure is not used in the analysis, but it is useful for visualizing the true data/MC agreement within the expected systematic uncertainties.

### 1. Decorrelation Example

To demonstrate that the  $\chi^2$  value of the decorrelated description is the same as the original covariance matrix formulation, consider the following example distribution  $\mathbf{x} \sim N(\boldsymbol{\mu}, \boldsymbol{\Sigma})$  which has only two normally distributed variables with means

$$\boldsymbol{\mu} = \begin{bmatrix} \mu_1 \\ \mu_2 \end{bmatrix} = \begin{bmatrix} 100 \\ 100 \end{bmatrix} \quad (\text{A6})$$

and covariance matrix

$$\boldsymbol{\Sigma} = \begin{bmatrix} \Sigma_{11} & \Sigma_{12} \\ \Sigma_{21} & \Sigma_{22} \end{bmatrix} = \begin{bmatrix} 200 & 200 \\ 200 & 500 \end{bmatrix} \quad (\text{A7})$$

The covariance matrix is constructed by defining fractional systematic uncertainties  $\sigma_1 = 0.1$ ,  $\sigma_2 = 0.2$ , correlation between the variables  $\rho = 1$ , and including a Poisson statistical variance in the diagonal elements. One can compute the conditional variance on  $x_1$  given that  $x_2 = \alpha$  using Eq. 8 as follows

$$\bar{\Sigma} = 200 - (200)\left(\frac{1}{500}\right)(200) = 200 - 80 = 120 \quad (\text{A8})$$

Similarly, using Eq. 7 one can compute the conditional mean  $\bar{\mu}$ , which is given by

$$\bar{\mu} = 100 + (200)\left(\frac{1}{500}\right)(\alpha - 100) = 60 + \left(\frac{2}{5}\right)\alpha \quad (\text{A9})$$

which results in two independent Gaussian distributions,  $x_1 \sim N(\bar{\mu}, \bar{\Sigma})$  and  $x_2 \sim N(\mu_2, \Sigma_{22})$ . Suppose that an observation of the multivariate Gaussian distribution results in the values

$$\mathbf{x} = \begin{bmatrix} x_1 \\ x_2 \end{bmatrix} = \begin{bmatrix} 120 \\ 150 \end{bmatrix} \quad (\text{A10})$$

A  $\chi^2$  test statistic can be computed using both forms of this distribution in order to verify that the behavior is identical. The standard method for computing  $\chi^2$  given a set of observations and covariance matrix is given by

$$\chi^2 = \boldsymbol{\Delta}^T \boldsymbol{\Sigma}^{-1} \boldsymbol{\Delta} \quad (\text{A11})$$

where the vector  $\boldsymbol{\Delta}$  is defined by

$$\boldsymbol{\Delta} = \mathbf{x} - \boldsymbol{\mu} = \begin{bmatrix} 120 - 100 \\ 150 - 100 \end{bmatrix} = \begin{bmatrix} 20 \\ 50 \end{bmatrix} \quad (\text{A12})$$

and the inverse covariance matrix has the form

$$\boldsymbol{\Sigma}^{-1} = \frac{1}{600} \begin{bmatrix} 5 & -2 \\ -2 & 2 \end{bmatrix} \quad (\text{A13})$$

Therefore, the test statistic computed from the method in Eq. 14 is given by

$$\chi^2 = \frac{1}{600} \begin{bmatrix} 20 & 50 \end{bmatrix} \begin{bmatrix} 5 & -2 \\ -2 & 2 \end{bmatrix} \begin{bmatrix} 20 \\ 50 \end{bmatrix} = 5 \quad (\text{A14})$$

In the case of independent random variables, a  $\chi^2$  test statistic can be computed by taking the sum over contributions from each variable such that

$$\chi^2 = \sum_i \frac{(x_i - \mu_i)^2}{\Sigma_i} \quad (\text{A15})$$

where  $x_i$  are observed variables,  $\mu_i$  are the expected values, and  $\Sigma_i$  are the independent variances for each variable. The conditional expected value for  $x_1$  is computed from Eq. 12 as follows

$$\bar{\mu} = 60 + \left(\frac{2}{5}\right)150 = 120 \quad (\text{A16})$$

Substituting into the  $\chi^2$  form from Eq. 18, one arrives at

$$\begin{aligned} \chi^2 &= \frac{(x_1 - \bar{\mu})^2}{\Sigma} + \frac{(x_2 - \mu_2)^2}{\Sigma_{22}} \\ &= \frac{(120 - 120)^2}{120} + \frac{(150 - 100)^2}{500} \\ &= \frac{0}{120} + \frac{50^2}{500} = 5 \end{aligned} \quad (\text{A17})$$

The identical value computed for  $\chi^2$  demonstrates that one can use the methods of conditional distributions to extract independent Gaussian distributions from an initially correlated multivariate Gaussian distribution.

- 
- [1] P. Adamson *et al.* (MINOS), arXiv:1710.06488 (2017).
  - [2] G. Cowan, K. Cranmer, E. Gross, and O. Vitells, Eur. Phys. J. C **71**, 1554 (2011).
  - [3] P. Adamson *et al.* (MINOS), Phys. Rev. Lett. **117**, 151803 (2016).
  - [4] T. Bohlen, F. Cerutti, M. Chin, A. Fasso, A. Ferrari, P. Ortega, A. Mairiani, P. R. Sala, G. Smirnov, and V. Vlachoudis, Nucl. Data Sheets **120**, 211 (2014).
  - [5] A. Ferrari, P. R. Sala, A. Fasso, and J. Ranft, CERN Report No. CERN-2005-010, 2005 (2005).
  - [6] P. Adamson *et al.*, Nucl. Instrum. Methods A **806**, 279 (2016).
  - [7] C. Alt *et al.* (NA49), Eur. Phys. J. C **49**, 897 (2007).
  - [8] L. Aliaga *et al.* (MINERvA), Phys. Rev. D **94**, 092005 (2016), [Addendum: Phys. Rev. D **95**, 039903 (2017)].
  - [9] L. Aliaga *et al.* (MINERvA), Nucl. Instrum. Methods A **743**, 130 (2014).
  - [10] B. Pontecorvo, Sov. Phys. JETP **26**, 984 (1968), [Zh. Eksp. Teor. Fiz. 53, 1717 (1967)].
  - [11] V. N. Gribov and B. Pontecorvo, Phys. Lett. **28B**, 493 (1969).
  - [12] Z. Maki, M. Nakagawa, and S. Sakata, Prog. Theor. Phys. **28**, 870 (1962).
  - [13] H. Harari and M. Leurer, Phys. Lett. B **181**, 123 (1986).
  - [14] S. Avvakumov *et al.* (CCFR/NuTeV), Nucl. Phys. Proc. Suppl. **78**, 232 (1999).
  - [15] P. S. Auchincloss *et al.* (CCFR), Z Phys C **48**, 411 (1990).
  - [16] I. E. Stockdale *et al.* (CCFR), Phys. Rev. Lett. **52**, 1384 (1984).
  - [17] J. Altegoer *et al.* (NOMAD), Nucl. Instrum. Methods A **404** (1998).
  - [18] A. Lebedev, Ph.D. thesis, Harvard University (2007).
  - [19] M. Campanella, A. Ferrari, P. R. Sala, and S. Vanini, CERN Report No. CERN-ATL-SOFT-99-004, 1999 (1999).
  - [20] S. Agostinelli *et al.*, Nucl. Instrum. Meth. **A506**, 250 (2003).
  - [21] J. Allison *et al.*, IEEE Trans. Nucl. Sci. **53**, 270 (2006).
  - [22] H. Gallagher, Nucl. Phys. Proc. Suppl. **112**, 188 (2002).
  - [23] T. Katori, AIP Conf. Proc. **1663**, 030001 (2015).
  - [24] A. A. Aguilar-Arevalo *et al.* (MiniBooNE), Phys. Rev. D **81**, 092005 (2010).
  - [25] J. Nieves, J. E. Amaro, and M. Valverde, Phys. Rev. C **70**, 055503 (2004), ; **72**, 019902 (2005) [Erratum].
  - [26] P. A. Rodrigues *et al.* (MINERvA), Phys. Rev. Lett. **116**, 071802 (2016).
  - [27] Z. Koba, H. Nielsen, and P. Olesen, Nucl. Phys. B **40**, 317 (1972).
  - [28] A. Cabrera *et al.* (MINOS), Nucl. Instrum. Methods A **609**, 106 (2009).
  - [29] R. Merenyi, Ph.D. thesis, Tufts University (1990).
  - [30] S. Dytman, H. Gallagher, and M. Kordosky, arXiv:0806.2119 (2008).
  - [31] J. S. Conway, in *Proceedings, PHYSTAT 2011 Workshop on Statistical Issues Related to Discovery Claims in Search Experiments and Unfolding, CERN, Geneva, Switzerland 17-20 January 2011* (2011) pp. 115–120, arXiv:1103.0354 [physics.data-an].
  - [32] N. Berger, (private communication) (2018).
  - [33] U. Katz, “Future neutrino telescopes in water and ice,” (2018).
  - [34] R. B. Patterson, *A Search for Muon Neutrino to Electron Neutrino Oscillations at  $\delta(m^2) > 0.1 \text{ eV}^2$* , Ph.D. thesis, Princeton U. (2007).
  - [35] F. James and M. Roos, Computer Physics Communications **10**, 343 (1975).
  - [36] G. L. Fogli *et al.*, Phys. Rev. D **86**, 013012 (2012).
  - [37] I. Esteban, M. C. Gonzalez-Garcia, M. Maltoni, I. Martinez-Soler, and T. Schwetz, JHEP **2017**, 87 (2017).
  - [38] S. Parke and M. Ross-Lonergan, Phys. Rev. D **93**, 113009 (2016).
  - [39] M. L. Eaton, *Multivariate Statistics: a Vector Space Approach* (John Wiley and Sons, 1983).
